# Supplementary material for: Safe Reinforcement Learning with Natural Language Constraints
Source: arXiv:2010.05150 source file (2021-08-04)
Supplement: Supplementary file 1 [file appendix_experiment.tex]

% !TEX root = neurips_2019.tex
\begin{center}
\Large
\textbf{Supplementary Material for \\ Accelerating Safe Reinforcement Learning \\ with Constraint-mismatched Policies}
\end{center}

\paragraph{Outline.} 
Supplementary material is outlined as follows. 
%
%Section \ref{appendix:prior_bound} provides lower and upper bounds on reward and cost performance when learning from the baseline policy.
%
Section \ref{sec:impact} discusses the impact of the proposed algorithm.
Section \ref{appendix:sec:theorem:h_D} details the proof of updating $h_D$ in Lemma \ref{theorem:h_D}.
Section \ref{appendix:proof_update_rule_1} describes the proof of analytical solution to \algname\ in Eq. (\ref{eq:P2CPO_final}).
Section \ref{appendix:sec:converge} gives the proof of finite-time guarantee of \algname\ in Theorem \ref{theorem:P2CPO_converge} and discuss the difference between the KL-divergence and 2-norm projections.
Section \ref{sec:appendix_experiment} assembles the additional experiment results to provide a detailed examination of the proposed algorithm compared to the baselines. These include:\\
\begin{itemize}
    \item evaluation of the discounted reward versus the cumulative undiscounted constraint cost to demonstrate that \algname\ achieves better reward performance with fewer cost constraint violations,
    \item evaluation of performance of \algname\ guided by baseline policies with different $J_C(\pi_B)$ to demonstrate that \algname\ safely learns from the baseline policies which need not satisfy the cost constraint,
    \item ablation studies of using a fixed $h_D$ in \algname\ to demonstrate the importance of using the dynamic $h_D$ to improve the reward and cost performance,
    \item comparison of \algname\ and other annealing approaches to demonstrate that \algname\ exploits the baseline policy effectively,
    \item comparison of \algname\ under the KL-divergence and the 2-norm projections to demonstrate that they converge to different stationary points,
    \item evaluation of using different initial values of $h^0_D$ to demonstrate that the selection of the initial value does not affect the performance of \algname\ drastically.
\end{itemize}{}
Section \ref{sec:appendix_experiment} also details the environment parameters, the architectures of policies, computational cost, infrastructure for computation and the instructions for executing the code.
Section \ref{appendix:human_policy} provides a procedure for getting a baseline human policy.
Finally, we fill the Machine Learning Reproducibility Checklist in Section \ref{appendix:sec:reproduce}.

\section{Impact of \algname}%(it is like abstract)
\label{sec:impact}
Many autonomous systems such as self-driving cars and autonomous robots are complex.
In order to deal with this complexity,
researchers are increasingly using reinforcement learning in conjunction with imitation learning for designing control policies.
%Leveraging the baseline policy from the previous application that has a similar configuration to the new application prevents from learning the policy from scratch.
%This allows us to deploy reinforcement learning systems on a large scale.
The more we can learn from a previous policy (\eg human demonstration, previous applications), the fewer resources (\eg time, energy, engineering effort, cost) we need to learn a new policy.
The proposed algorithm could be applied in many fields where learning a policy can take advantage of prior applications while providing assurances for the consideration of fairness, safety, or other costs.
For example, in a dialogue system where an agent is intended to converse with a human, the agent should safely learn from human preferences while avoiding producing biased or offensive responses.
In addition, in the self-driving car domain where an agent learns a driving policy, the agent should safely learn from human drivers while avoiding a crash. 
Moreover, in the personalized robotic assistant setting where an agent learns from human demonstration, the agent should carefully imitate humans without damaging itself or causing harm to nearby humans.
These examples highlight the potential impact of the proposed algorithm for accelerating safe reinforcement learning by adapting prior knowledge.
This can open the door to advances in lifelong learning and adaptation of agents to different contexts. 
%
%and dynamic environments, while subject to safety limitations.

%
One deficiency of the proposed algorithm is that the agent still experiments with cost constraint violation when learning control policies.
This is because that any learning-based system needs to experiment with various actions to find a constraint-satisfying policy.
Even though the agent does not violate the safety constraints during the learning phase, any change or perturbation of the environment that was not envisioned at the time of programming or training may lead to a catastrophic failure during run-time.
These systems cannot guarantee that sensor inputs will not induce undesirable consequences, nor can the systems adapt and support safety in situations in which new objectives are created. 
This creates huge concerns in safety-critical applications such as self-driving vehicles and personalized chatbot system.
% 
%Nonetheless, being able to apply knowledge to new situations and learn fast, subject to safety constraints, can support assurance in the operation of the system when the system and environment evolve.
%

%
This raises several questions:
What human-agent communication is needed to bring humans in the loop to increase safety guarantees for the autonomous system? 
How can trust and safety constraints be incorporated into the planning and control processes?
How can one effectively identify unsafe plans of the baseline policy?
We believe this paper will encourage future work to develop rigorous design and analysis tools for continual safety assurance in conjunction with using baseline policies from previous applications. 

\section{Proof of Updating $h_D$ in Lemma \ref{theorem:h_D}}
\label{appendix:sec:theorem:h_D}

\begin{proof}
Based on Theorem 1 in \cite{achiam2017constrained}, for any two policies $\pi$ and $\pi'$ we have
\begin{align}
    &J_{C}(\pi') - J_{C}(\pi)\geq \frac{1}{1-\gamma}\E_{\substack{s\sim d^{\pi}\\ a\sim \pi'}}\Big[A^{\pi}_{C}(s,a)-\frac{2\gamma\epsilon^{\pi'}_{C}}{1-\gamma}\sqrt{\frac{1}{2}\KL(\pi'(s)||\pi(s))}\Big]\nonumber \\ 
    \Rightarrow\quad&
    \frac{2\gamma\epsilon^{\pi'}_C}{(1-\gamma)^2}\E_{\substack{s\sim d^{\pi}}}\Big[\sqrt{\frac{1}{2}\KL(\pi'(s)||\pi(s))}\Big]\geq -J_{C}(\pi')+J_{C}(\pi)+\frac{1}{1-\gamma}\E_{\substack{s\sim d^{\pi}\\ a\sim \pi'}}\Big[A^{\pi}_{C}(s,a)\Big]\nonumber \\ 
    \Rightarrow\quad&\frac{2\gamma\epsilon^{\pi'}_C}{(1-\gamma)^2}\E_{\substack{s\sim d^{\pi}}}\Big[\sqrt{\frac{1}{2}\KL(\pi'(s)||\pi(s))}\Big]\geq -J_{C}(\pi')+J_{C}(\pi)\nonumber \\ 
    \Rightarrow\quad&\frac{\sqrt{2}\gamma\epsilon^{\pi'}_C}{(1-\gamma)^2}\sqrt{\E_{\substack{s\sim d^{\pi}}}\Big[\KL(\pi'(s)||\pi(s))\Big]}\geq -J_{C}(\pi')+J_{C}(\pi)\nonumber \\ 
    \Rightarrow\quad&\E_{\substack{s\sim d^{\pi}}}\Big[\KL(\pi'(s)||\pi(s))\Big]\geq \frac{(1-\gamma)^4(-J_{C}(\pi')+J_{C}(\pi))^2}{2\gamma^2{\epsilon^{\pi'}_C}^2}.
    \label{eq:appendix_B_1}
\end{align}
The fourth inequality follows from Jensen's inequality. 
We then define $\varphi(\pi(s))\doteq\sum_i \pi(a(i)|s)\log \pi(a(i)|s).$
By Three-point Lemma~\cite{chen1993convergence}, for any three policies $\pi, \pi',$ and $\hat{\pi}$ we have
\begin{align}
    \E_{\substack{s\sim d^{\pi}}}\Big[\KL(\pi'(s)||\hat{\pi}(s))\Big]= \E_{\substack{s\sim d^{\pi}}}\Big[\KL(\pi'(s)||{\pi(s)})\Big]+ \E_{\substack{s\sim d^{\pi}}}\Big[\KL(\pi(s)||\hat{\pi}(s))\Big]\nonumber \\ 
    -\E_{s\sim d^{\pi}}\Big[(\nabla\varphi(\hat{\pi}(s))-\nabla\varphi(\pi(s)))^T(\pi'(s)-\pi(s))\Big].
    \label{eq:appendix_B_2}
\end{align}

\begin{figure*}[t]
\vspace{-3mm}
\centering
\subfloat[]{
\includegraphics[width=0.36\linewidth]{figure/relaxing_2_proof.pdf}}
\subfloat[]{
\includegraphics[width=0.33\linewidth]{figure/relaxing_1_proof.pdf}}
\caption{
\textbf{(a)} Illustrating when $\pi_B$ is \textit{outside} the cost constraint set. 
%
%$\pi_{boundary}$ is the policy with $J_C(\pi_{boundary})=h_C.$ 
%
%We aim to bound $h_D^{k+1}$ (\ie the KL-divergence between $\pi_{boundary}$ and $\pi_B$) by using the threshold $h_D^k.$
%
\textbf{(b)} Illustrating when $\pi_B$ is \textit{inside} the cost constraint set. 
$\pi_{boundary}$ is the policy with $J_C(\pi_{boundary})=h_C.$ 
We aim to bound $h_D^{k+1}$ (\ie the KL-divergence between $\pi_{boundary}$ and $\pi_B$) by using $h_D^k.$
}
\vspace{-3mm}
\label{fig:p2cpo_appendix}
\vspace{-3mm}
%\end{mdframed}
\end{figure*}

Let $\pi_{boundary}$ denote a policy satisfying~$J_C(\pi_{boundary})=h_C$ (\ie $\pi_{boundary}$ is in the boundary of the set of the policies which satisfy the cost constraint $J_C(\pi)\leq h_C$).
Let $\pi'=\pi_{boundary}, \hat{\pi}=\pi_B$ and $\pi=\pi^{k}$ in Eq. (\ref{eq:appendix_B_1}) and Eq. (\ref{eq:appendix_B_2}) (this is illustrated in Fig. \ref{fig:p2cpo_appendix}).
Then we have 
\begin{align}
    &~\E_{\substack{s\sim d^{\pi^k}}}\Big[\KL(\pi_{boundary}(s)||\pi_B(s))\Big]-\E_{\substack{s\sim d^{\pi^k}}}\Big[\KL(\pi^{k}(s)||\pi_B(s))\Big]
    \nonumber \\ = &~
     \E_{\substack{s\sim d^{\pi^k}}}\Big[\KL(\pi_{boundary}(s)||{\pi^k(s)})\Big]\nonumber\\
     &\quad\quad\quad-\E_{s\sim d^{\pi^k}}\Big[(\nabla\varphi(\pi_B(s))-\nabla\varphi(\pi^k(s)))^T(\pi_{boundary}(s)-\pi^{k}(s))\Big]\nonumber \\ 
     \geq &~ \frac{(1-\gamma)^4(-J_{C}(\pi_{boundary})+J_{C}(\pi^{k}))^2}{2\gamma^2{\epsilon^{\pi'}_C}^2}\nonumber\\
     &\quad\quad\quad-\E_{s\sim d^{\pi^k}}\Big[(\nabla\varphi(\pi_B(s))-\nabla\varphi(\pi^k(s)))^T(\pi_{boundary}(s)-\pi^{k}(s))\Big]
     \nonumber \\ = &~ \frac{(1-\gamma)^4(-h_C+J_{C}(\pi^k))^2}{2\gamma^2{\epsilon^{\pi'}_C}^2}
     \nonumber\\
     &\quad\quad\quad-\E_{s\sim d^{\pi^k}}\Big[(\nabla\varphi(\pi_B(s))-\nabla\varphi(\pi^k(s)))^T(\pi_{boundary}(s)-\pi^{k}(s))\Big]\nonumber \\ =&~\mathcal{O}\Big(\big(-h_C + J_{C}(\pi^k)\big)^2\Big),\label{eq:bound_for_hc_appendix}
\end{align}
where $J_C(\pi_{boundary})=h_C.$

For the first case in Fig. \ref{fig:p2cpo_appendix}(a), we would like to have $\mathcal{U}_1\cap \mathcal{U}_2^{k+1}\neq \emptyset$~(feasibility). 
For the second case in Fig. \ref{fig:p2cpo_appendix}(b), we would like to have $\mathcal{U}_2^{k+1}\cap\partial\mathcal{U}_1\neq\emptyset$~(exploration).
These implies that the policy in step $k+1$ is $\pi_{boundary}$ which satisfies $\mathcal{U}_1\cap \mathcal{U}_2^{k+1}\neq \emptyset$ and $\mathcal{U}_2^{k+1}\cap\partial\mathcal{U}_1\neq\emptyset.$
Now let $h_D^{k+1}\doteq \E_{\substack{s\sim d^{\pi^k}}}\Big[\KL(\pi_{boundary}(s)||\pi_B(s))\Big]$ and 
$h_D^k \doteq \E_{\substack{s\sim d^{\pi^k}}}[\KL(\pi^k(s)||\pi_B(s))].$ 
Then Eq. \ref{eq:bound_for_hc_appendix} implies 
\begin{align}
   h^{k+1}_D \geq \mathcal{O}\Big(\big(-h_C + J_{C}(\pi^k)\big)^2\Big) + h_D^k. \nonumber
\end{align}
%Note that $\mathcal{O}(\cdot)$ absorbs the error of bounding the inequality $\E_{\substack{s\sim d^{\pi^k}}}\Big[\KL(\pi^{k}(s)||\pi_B(s))\Big]\leq h^k_D.$ 
\end{proof}
Lemma~\ref{theorem:h_D} theoretically ensures $h_D$ is large enough to guarantee feasibility and exploration of the agent.
Note that we do not provide guarantees for finding an optimal policy.
This requires additional assumptions on the objective function (\eg convexity).

In addition, the goal of this paper is to understand and analyze how to effectively exploit a baseline policy in constrained RL.
Without such an analysis,
we are not confident in deploying SPACE in real applications.
Furthermore, the question of safely using baseline policies has a practical potential.
It is less studied by prior work \cite{achiam2017constrained,chow2019lyapunov,tessler2018reward,yang2020projection}.

\section{Proof of Analytical Solution to \algname\ in Eq. (\ref{eq:P2CPO_final})}
\label{appendix:proof_update_rule_1}

We first approximate the three stages in \algname\ using the following approximations.

\parab{Step 1.} 
Approximating Eq. (\ref{eq:P2CPO_firstStep}) yields
\begin{align}\textstyle
    \vtheta^{k+\frac{1}{3}} = \argmax\limits_{\vtheta}~ {\vg^{k}}^{T}(\vtheta-\vtheta^{k})\quad\text{s.t.}&~\frac{1}{2}(\vtheta-\vtheta^{k})^{T}\mF^{k}(\vtheta-\vtheta^{k})\leq \delta.
    \label{eq:update1}
\end{align}
\parab{Step 2 and Step 3.}
% Second, if the projections are defined in the parameter space, we directly use the 2-norm projection.
%
%On the other hand, if the projections are defined in the probability space, we use the KL-divergence projection, which is approximated through a second order Taylor expansion.
%
Approximating Eq. (\ref{eq:P2CPO_secondStep}) and (\ref{eq:P2CPO_thridStep}), similarly yields
%at $\pi^{k+\frac{1}{3}}$ and $\pi^{k+\frac{2}{3}}$
%And we approximate the constraints in Eq. (\ref{eq:P2CPO_secondStep}) and (\ref{eq:P2CPO_thridStep}) by a first order Taylor expansion.
\begin{align}\textstyle
    \vtheta^{k+\frac{2}{3}}=\argmin\limits_{\vtheta}&~\frac{1}{2}(\vtheta-{\vtheta}^{k+\frac{1}{3}})^{T}\mL(\vtheta-{\vtheta}^{k+\frac{1}{3}}) \quad \text{s.t.}~{\va^{ k}}^{T}(\vtheta-\vtheta^{k})+b^{k}\leq 0, \label{eq:update2}\\
    \vtheta^{k+1} = \argmin\limits_{\vtheta}&~\frac{1}{2}(\vtheta-{\vtheta}^{k+\frac{2}{3}})^{T}\mL(\vtheta-{\vtheta}^{k+\frac{2}{3}})\quad\text{s.t.}~{\vc^{ k}}^{T}(\vtheta-\vtheta^{k})+d^{k}\leq 0,
    \label{eq:update3}
\end{align}
where $\mL=\mI$ for the 2-norm projection and $\mL=\mF^{k}$ for the KL-divergence projection.

\begin{proof}
For the first problem in Eq. (\ref{eq:update1}), since $\mF^k$ is the Fisher Information matrix, it is positive semi-definite.
Hence it is a convex program with quadratic inequality constraints.
If the primal problem has a feasible point,
then Slater’s condition is satisfied and strong duality holds. 
Let $\vtheta^{*}$ and $\lambda^*$ denote the solutions to the primal and dual problems, respectively.
In addition, the primal objective function  is continuously differentiable.
Hence the Karush-Kuhn-Tucker (KKT) conditions are necessary and sufficient for the optimality of $\vtheta^{*}$ and $\lambda^*.$
We now form the Lagrangian:
\[
\mathcal{L}(\vtheta,\lambda)=-{\vg^k}^{T}(\vtheta-\vtheta^{k})+\lambda\Big(\frac{1}{2}(\vtheta-\vtheta^{k})^{T}\mF^k(\vtheta-\vtheta^{k})- \delta\Big).
\]
And we have the following KKT conditions:
\begin{align}
   -\vg^k + \lambda^*\mF^k\vtheta^{*}-\lambda^*\mF^k\vtheta^{k}=0~~~~&~~~\nabla_\vtheta\mathcal{L}(\vtheta^{*},\lambda^{*})=0 \label{KKT_1}\\
   \frac{1}{2}(\vtheta^{*}-\vtheta^{k})^{T}\mF^k(\vtheta^{*}-\vtheta^{k})- \delta=0~~~~&~~~\nabla_\lambda\mathcal{L}(\vtheta^{*},\lambda^{*})=0 \label{KKT_2}\\
    \frac{1}{2}(\vtheta^{*}-\vtheta^{k})^{T}\mF^k(\vtheta^{*}-\vtheta^{k})-\delta\leq0~~~~&~~~\text{primal constraints}\label{KKT_3}\\
   \lambda^*\geq0~~~~&~~~\text{dual constraints}\label{KKT_4}\\
   \lambda^*\Big(\frac{1}{2}(\vtheta^{*}-\vtheta^{k})^{T}\mF^k(\vtheta^{*}-\vtheta^{k})-\delta\Big)=0~~~~&~~~\text{complementary slackness}\label{KKT_5}
\end{align}
By Eq.~(\ref{KKT_1}), we have $\vtheta^{*}=\vtheta^k+\frac{1}{\lambda^*}{\mF^k}^{-1}\vg^k.$ 
And by plugging Eq.~(\ref{KKT_1}) into Eq.~(\ref{KKT_2}), 
we have $\lambda^*=\sqrt{\frac{{\vg^k}^T{\mF^k}^{-1}\vg^k}{2\delta}}.$
Hence we have a solution
\begin{align}
\vtheta^{k+\frac{1}{3}}=\vtheta^{*}=\vtheta^k+\sqrt{\frac{2\delta}{{\vg^k}^T{\mF^k}^{-1}\vg^k}}{\mF^k}^{-1}\vg^k, \label{KKT_First}    
\end{align}
which also satisfies Eq.~(\ref{KKT_3}), Eq.~(\ref{KKT_4}), and Eq.~(\ref{KKT_5}).
For the second problem in Eq. (\ref{eq:update2}), we follow the same procedure for the first problem to form the Lagrangian:
\begin{align}
\mathcal{L}(\vtheta,\lambda)=\frac{1}{2}(\vtheta-{\vtheta}^{k+\frac{1}{3}})^{T}\mL(\vtheta-{\vtheta}^{k+\frac{1}{3}})+\lambda({\va^k}^T(\vtheta-\vtheta^k)+b^k). \nonumber
\end{align}
And we have the following KKT conditions: 
\begin{align}
  \mL\vtheta^*-\mL\vtheta^{k+\frac{1}{3}}+\lambda^*\va^k=0~~~~&~~~\nabla_\vtheta\mathcal{L}(\vtheta^{*},\lambda^{*})=0 \label{KKT_6}\\
   {\va^k}^T(\vtheta^*-\vtheta^k)+b^k=0~~~~&~~~\nabla_\lambda\mathcal{L}(\vtheta^{*},\lambda^{*})=0 \label{KKT_7}\\
    {\va^k}^T(\vtheta^*-\vtheta^k)+b^k\leq0~~~~&~~~\text{primal constraints}\label{KKT_8}\\
   \lambda^*\geq0~~~~&~~~\text{dual constraints}\label{KKT_9}\\
   \lambda^*({\va^k}^T(\vtheta^*-\vtheta^k)+b^k)=0~~~~&~~~\text{complementary slackness}\label{KKT_10}
\end{align}
By Eq.~(\ref{KKT_6}), we have $\vtheta^{*}=\vtheta^{k}+\lambda^*\mL^{-1}\va^k.$ 
And by plugging Eq.~(\ref{KKT_6}) into Eq.~(\ref{KKT_7}) and Eq.~(\ref{KKT_9}), 
we have $\lambda^*=\max(0,\frac{{\va^k}^T(\vtheta^{k+\frac{1}{3}}-\vtheta^{k})+b^k}{\va^k\mL^{-1}\va^k}).$
Hence we have a solution
\begin{align}
\vtheta^{k+\frac{2}{3}}=\vtheta^{*}=\vtheta^{k+\frac{1}{3}}-\max(0,\frac{{\va^k}^T(\vtheta^{k+\frac{1}{3}}-\vtheta^k)+b^k}{{\va^k}^T\mL^{-1}{\va^k}^T})\mL^{-1}\va^k,\label{KKT_Second}
\end{align}
which also satisfies Eq.~(\ref{KKT_8}) and Eq.~(\ref{KKT_10}). 
For the third problem in Eq. (\ref{eq:update3}), instead of doing the projection on $\pi^{k+\frac{2}{3}}$ which is the intermediate policy obtained in the second step, we project the policy $\pi^{k+\frac{1}{3}}$ onto the cost constraint.
This allows us to compute the projection without too much computational cost.
We follow the same procedure for the first and second problems to form the Lagrangian:
\begin{align}
\mathcal{L}(\vtheta,\lambda)=\frac{1}{2}(\vtheta-{\vtheta}^{k+\frac{1}{3}})^{T}\mL(\vtheta-{\vtheta}^{k+\frac{1}{3}})+\lambda({\vc^k}^T(\vtheta-\vtheta^k)+d^k). \nonumber
\end{align}
And we have the following KKT conditions: 
\begin{align}
  \mL\vtheta^*-\mL\vtheta^{k+\frac{1}{3}}+\lambda^*\vc^k=0~~~~&~~~\nabla_\vtheta\mathcal{L}(\vtheta^{*},\lambda^{*})=0 \label{KKT_6_C}\\
   {\vc^k}^T(\vtheta^*-\vtheta^k)+d^k=0~~~~&~~~\nabla_\lambda\mathcal{L}(\vtheta^{*},\lambda^{*})=0 \label{KKT_7_C}\\
    {\vc^k}^T(\vtheta^*-\vtheta^k)+d^k\leq0~~~~&~~~\text{primal constraints}\label{KKT_8_C}\\
   \lambda^*\geq0~~~~&~~~\text{dual constraints}\label{KKT_9_C}\\
   \lambda^*({\vc^k}^T(\vtheta^*-\vtheta^k)+d^k)=0~~~~&~~~\text{complementary slackness}\label{KKT_10_C}
\end{align}
By Eq.~(\ref{KKT_6_C}), we have $\vtheta^{*}=\vtheta^{k}+\lambda^*\mL^{-1}\vc^k.$ 
And by plugging Eq.~(\ref{KKT_6_C}) into Eq.~(\ref{KKT_7_C}) and Eq.~(\ref{KKT_9_C}), 
we have $\lambda^*=\max(0,\frac{{\vc^k}^T(\vtheta^{k+\frac{1}{3}}-\vtheta^{k})+d^k}{\vc^k\mL^{-1}\vc^k}).$
Hence we have a solution
\begin{align}
\vtheta^{k+1}=\vtheta^{*}=\vtheta^{k+\frac{1}{3}}-\max(0,\frac{{\vc^k}^T(\vtheta^{k+\frac{1}{3}}-\vtheta^{k})+d^k}{{\vc^k}^T\mL^{-1}{\vc^k}^T})\mL^{-1}\vc^k.\label{KKT_Thrid}
\end{align}

Hence by combining Eq.~(\ref{KKT_First}), Eq.~(\ref{KKT_Second}) and Eq.~(\ref{KKT_Thrid}), we have 
\begin{align}
\vtheta^{k+1}=\vtheta^{k}+\sqrt{\frac{2\delta}{{\vg^k}^T{\mF^k}^{-1}\vg^k}}{\mF^k}^{-1}\vg^k
-&\max(0,\frac{\sqrt{\frac{2\delta}{{\vg^k}^T{\mF^k}^{-1}\vg^k}}{\va^k}^{T}{\mF^k}^{-1}\vg^k+b^k}{{\va^k}^T\mL^{-1}\va^k})\mL^{-1}\va^k \nonumber \\ -&\max(0,\frac{\sqrt{\frac{2\delta}{{\vg^k}^T{\mF^k}^{-1}\vg^k}}{\vc^k}^{T}{\mF^k}^{-1}\vg^k+d^k}{{\vc^k}^T\mL^{-1}\vc^k})\mL^{-1}\vc^k.\nonumber
\end{align}
\end{proof}

\section{Proof of Finite-Time Guarantee of \algname\ in Theorem \ref{theorem:P2CPO_converge}}
\label{appendix:sec:converge}
We now describe the reason for choosing two variants of $\epsilon$-FOSP under two possible projections.
Let $\eta^k_R$ denote the step size for the reward, $\eta^k_D$ denote the step size for the divergence cost, and $\eta^k_C$ denote the step size for the constraint cost.
Without loss of generality, under the KL-divergence projection, at step $k+1$ \algname\ does
\begin{align}
    \vtheta^{k+1}=\vtheta^{k}+\eta^k_R{\mF^{k}}^{-1}\vg^{k}-\eta^k_D{\mF^{k}}^{-1}\va^{k}-\eta^k_C{\mF^{k}}^{-1}\vc^{k}.\nonumber
\end{align}
Similarly, under the 2-norm projection, at step $k+1$ \algname\ does
\begin{align}
    \vtheta^{k+1}=\vtheta^{k}+\eta^k_R{\mF^{k}}\vg^{k}-\eta^k_D\va^{k}-\eta^k_C\vc^{k}.\nonumber
\end{align}
With this definition, we have the following Lemma.
\begin{lemma}[\textbf{Stationary Points for \algname}]
\label{def_fosp}
 Under the KL-divergence projection, \algname\ converges to a stationary point $\vtheta^*$ satisfying
 \begin{align}
     \eta^*_R\vg^*=\eta^*_D\va^*+\eta^*_C\vc^*.\nonumber
 \end{align}
  Under the 2-norm projection, \algname\ converges to a stationary point $\vtheta^*$ satisfying
 \begin{align}
     \eta^*_R\vg^*={\mF^*}(\eta^*_D\va^*+\eta^*_C\vc^*).\nonumber
 \end{align}
\end{lemma}
\begin{proof}
 Under the KL-divergence projection, by using the definition of a stationary point we have
 \begin{align}
     &\vtheta^{*}=\vtheta^{*}+\eta^*_R{\mF^{*}}^{-1}\vg^{*}-\eta^*_D{\mF^{*}}^{-1}\va^{*}-\eta^*_C{\mF^{*}}^{-1}\vc^{*}\nonumber\\
     \Rightarrow\quad& \eta^*_R{\mF^{*}}^{-1}\vg^{*}=\eta^*_D{\mF^{*}}^{-1}\va^{*}+\eta^*_C{\mF^{*}}^{-1}\vc^{*}\nonumber\\
     \Rightarrow\quad&\eta^*_R\vg^{*}=\eta^*_D\va^{*}+\eta^*_C\vc^{*}.\nonumber
 \end{align}
 Under the 2-norm projection, by using the definition of a stationary point we have
  \begin{align}
     &\vtheta^{*}=\vtheta^{*}+\eta^*_R{\mF^{*}}^{-1}\vg^{*}-\eta^*_D\va^{*}-\eta^*_C\vc^{*}\nonumber\\
     \Rightarrow\quad& \eta^*_R{\mF^{*}}^{-1}\vg^{*}=\eta^*_D\va^{*}+\eta^*_C\vc^{*}\nonumber\\
     \Rightarrow\quad&\eta^*_R\vg^{*}={\mF^{*}}(\eta^*_D\va^{*}+\eta^*_C\vc^{*}).\nonumber
 \end{align}
\end{proof}
Hence Lemma \ref{def_fosp} motivates the need for defining two variants of FOSP.

Before proving Theorem \ref{theorem:P2CPO_converge}, we need the following Lemma. 
Define $\mathcal{P}^{\mL}_{\mathcal{C}}(\vtheta)\doteq\argmin\limits_{\vtheta'\in\mathcal{C}}\|\vtheta-\vtheta'\|^2_\mL=\argmin\limits_{\vtheta'\in\mathcal{C}}{(\vtheta-\vtheta')}^T\mL(\vtheta-\vtheta'),$ and $\mL=\mF^k$ under the KL-divergence projection, and $\mL=\mI$ under the 2-norm projection.
\begin{lemma}[\textbf{Contraction of Projection}~\cite{yang2020projection}]
\label{lemma:projecion_appendix}
For any $\vtheta,$ $\vtheta^{*}=\mathcal{P}^{\mL}_{\mathcal{C}}(\vtheta)$ if and only if ${(\vtheta-\vtheta^*)}^T\mL(\vtheta'-\vtheta^*)\leq0, \forall\vtheta'\in\mathcal{C}.$
\end{lemma}
\begin{proof}

$(\Rightarrow)$ Let $\vtheta^{*}=\mathcal{P}^{\mL}_{\mathcal{C}}(\vtheta)$ for a given $\vtheta \not\in\mathcal{C},$ $\vtheta'\in\mathcal{C}$ be such that $\vtheta'\neq\vtheta^*,$ and $\alpha\in(0,1).$ Then we have
\begin{align}
    \|\vtheta-\vtheta^*\|^2_\mL&\leq\|\vtheta-\big(\vtheta^*+\alpha(\vtheta'-\vtheta^*)\big)\|^2_\mL \nonumber\\
    &=\|\vtheta-\vtheta^*\|^2_\mL + \alpha^2\|\vtheta'-\vtheta^*\|^2_\mL-2\alpha(\vtheta-\vtheta^*)^T\mL(\vtheta'-\vtheta^*) \nonumber\\
    \Rightarrow (\vtheta-\vtheta^*)^T\mL(\vtheta'-\vtheta^*)&\leq \frac{\alpha}{2}\|\vtheta'-\vtheta^*\|^2_\mL. \label{eq:appendix_lemmaD1_0}
\end{align}
Since the right hand side of Eq. (\ref{eq:appendix_lemmaD1_0}) can be made arbitrarily small for a given $\alpha$, we have
\[
(\vtheta-\vtheta^*)^T\mL(\vtheta'-\vtheta^*)\leq0, \forall\theta'\in\mathcal{C}.
\]

$(\Leftarrow)$ Let $\vtheta^*\in\mathcal{C}$ be such that $(\vtheta-\vtheta^*)^T\mL(\vtheta'-\vtheta^*)\leq0, \forall\theta'\in\mathcal{C}.$ We show that $\vtheta^*$ must be the optimal solution. Let $\vtheta'\in\mathcal{C}$ and $\vtheta'\neq\vtheta^*.$ Then we have
\begin{align}
    \|\vtheta-\vtheta'\|^2_\mL - \|\vtheta-\vtheta^*\|^2_\mL &=\|\vtheta-\vtheta^*+\vtheta^*-\vtheta'\|^2_\mL -\|\vtheta-\vtheta^*\|^2_\mL \nonumber\\
    &=\|\vtheta-\vtheta^*\|^2_\mL + \|\vtheta'-\vtheta^*\|^2_\mL - 2(\vtheta-\vtheta^*)^T\mL(\vtheta'-\vtheta^*) - \|\vtheta-\vtheta^*\|^2_\mL\nonumber\\
    &>0\nonumber\\
    \Rightarrow \|\vtheta-\vtheta'\|^2_\mL&>\|\vtheta-\vtheta^*\|^2_\mL.\nonumber
\end{align}
Hence, $\vtheta^*$ is the optimal solution to the optimization problem, and $\vtheta^*=\mathcal{P}^{\mL}_{\mathcal{C}}(\vtheta).$
\end{proof}

We now prove Theorem \ref{theorem:P2CPO_converge}. 
Without loss of generality, on each learning episode \algname\ updates the reward followed by the alternation of two projections onto the constraint sets (region around $\pi_B$ and the cost constraint set):
\begin{align}
  &\vtheta^{k+\frac{1}{3}} 
  =\vtheta^k-\eta^{k} \mF^{-1}\nabla f(\vtheta^k),~\vtheta^{k+\frac{2}{3}}=\mathcal{P}_{\mathcal{C}_2}(\vtheta^{k+\frac{1}{3}}),~
    \vtheta^{k+1}=\mathcal{P}_{\mathcal{C}_1}(\vtheta^{k+\frac{2}{3}}),\text{if $\vtheta^{k}\in\mathcal{C}_2,$}\nonumber\\
      &\vtheta^{k+\frac{1}{3}} 
      =\vtheta^k-\eta^{k} \mF^{-1}\nabla f(\vtheta^k),~ \vtheta^{k+\frac{2}{3}}=\mathcal{P}_{\mathcal{C}_1}(\vtheta^{k+\frac{1}{3}}),~
    \vtheta^{k+1}=\mathcal{P}_{\mathcal{C}_2}(\vtheta^{k+\frac{2}{3}}),\text{if $\vtheta^{k}\in\mathcal{C}_1,$}\nonumber
\end{align}
where $\eta^{k}$ is the step size at step $k.$

\begin{proof}
\textbf{\algname\ under the KL-divergence projection converges to an $\epsilon$-FOSP.} Based on Lemma \ref{lemma:projecion_appendix} under the KL-divergence projection, and setting $\vtheta=\vtheta^k-\eta^k{\mF^k}^{-1}\nabla f(\vtheta^k),$ $\vtheta^*=\vtheta^{k+\frac{2}{3}}$ and $\vtheta'=\vtheta^k,$ we have 
\begin{align}
   &(\vtheta^{k}-\vtheta^{k+\frac{2}{3}})^T\mF^k(\vtheta^k-\eta^k{\mF^k}^{-1}\nabla f(\vtheta^k)-\vtheta^{k+\frac{2}{3}})\leq0\nonumber\\
   \Rightarrow\quad&\nabla f(\vtheta^k)^T(\vtheta^{k+\frac{2}{3}}-\vtheta^{k})\leq - \frac{1}{\eta^k}{(\vtheta^{k+\frac{2}{3}}-\vtheta^{k})^T}\mF^k(\vtheta^{k+\frac{2}{3}}-\vtheta^{k}).
   \label{eq:appendix_converge_0}
\end{align}
Based on the $L$-Lipschitz continuity of gradients and Eq. (\ref{eq:appendix_converge_0}), we have 
\begin{align}
f(\vtheta^{k+\frac{2}{3}})& \leq  f(\vtheta^{k})+{\nabla f(\vtheta^k)^T}(\vtheta^{k+\frac{2}{3}}-\vtheta^{k})+\frac{L}{2}{\|\vtheta^{k+\frac{2}{3}}-\vtheta^{k}\|^2} \nonumber \\ 
&\leq f(\vtheta^{k}) - \frac{1}{\eta^k}{(\vtheta^{k+\frac{2}{3}}-\vtheta^{k})^T}\mF^k(\vtheta^{k+\frac{2}{3}}-\vtheta^{k})+\frac{L}{2}{\|\vtheta^{k+\frac{2}{3}}-\vtheta^{k}\|^2}\nonumber \\
&= f(\vtheta^{k})-\frac{L}{2}{\|\vtheta^{k+\frac{2}{3}}-\vtheta^{k}\|^2}-{\nabla f(\vtheta^{k+\frac{2}{3}})^T}(\vtheta^{k+1}-\vtheta^{k+\frac{2}{3}})-\frac{L}{2}{\|\vtheta^{k+1}-\vtheta^{k+\frac{2}{3}}\|^2},
\label{eq:thrm4_1_1}
\end{align}
where the equality follows by setting $\delta$ (\ie the size of the trust region) such that 
\[
\eta^k=\frac{(\vtheta^{k+\frac{2}{3}}-\vtheta^{k})^T\mF^k(\vtheta^{k+\frac{2}{3}}-\vtheta^{k})}{L\|\vtheta^{k+\frac{2}{3}}-\vtheta^{k}\|^2+\nabla f(\vtheta^{k+\frac{2}{3}})^T(\vtheta^{k+1}-\vtheta^{k+\frac{2}{3}})+\frac{L}{2}\|\vtheta^{k+1}-\vtheta^{k+\frac{2}{3}}\|^2}.
\]
Again, based on Lemma \ref{lemma:projecion_appendix}, for $\vtheta\in\mathcal{C}_2$ we have 
\begin{align}
    &{(\vtheta^{k}-\eta^k{\mF^k}^{-1}\nabla f(\vtheta^k)-\vtheta^{k+\frac{2}{3}})}\mF^k(\vtheta-\vtheta^{k+\frac{2}{3}})\leq0 \nonumber \\ 
    \Rightarrow\quad&(-\eta^k{\mF^k}^{-1}\nabla f(\vtheta^k))^T\mF^k(\vtheta-\vtheta^{k+\frac{2}{3}})\leq-(\vtheta^{k}-\vtheta^{k+\frac{2}{3}})^T\mF^k(\vtheta-\vtheta^{k+\frac{2}{3}})\nonumber \\ 
    \Rightarrow\quad&\nabla f(\vtheta^k)^T(\vtheta-\vtheta^{k+\frac{2}{3}}) \geq \frac{1}{\eta^k}(\vtheta^{k}-\vtheta^{k+\frac{2}{3}})^T\mF^k(\vtheta-\vtheta^{k+\frac{2}{3}})\nonumber \\ 
    \Rightarrow\quad& \nabla f(\vtheta^k)^T\vtheta\geq\nabla f(\vtheta^k)^T\vtheta^{k+\frac{2}{3}}+\frac{1}{\eta^k}(\vtheta^k-\vtheta^{k+\frac{2}{3}})^T\mF^k(\vtheta-\vtheta^{k+\frac{2}{3}})\nonumber \\ 
    \Rightarrow\quad&f(\vtheta^k)^T(\vtheta-\vtheta^{k})\geq\nabla f(\vtheta^k)^T(\vtheta^{k+\frac{2}{3}}-\vtheta^{k})+\frac{1}{\eta^k}(\vtheta^k-\vtheta^{k+\frac{2}{3}})^T\mF^k(\vtheta-\vtheta^{k+\frac{2}{3}})\nonumber \\ 
    & \geq -\|\nabla f(\vtheta^k)\|\|\vtheta^{k+\frac{2}{3}}-\vtheta^{k}\|-\frac{1}{\eta^k}\|\vtheta^{k+\frac{2}{3}}-\vtheta^{k}\|\|\mF^k\|\|\vtheta-\vtheta^{k+\frac{2}{3}}\|\nonumber \\ 
    & \geq -\big(G+\frac{D\sigma_1(\mF^k)}{\eta^k}\big)\|\vtheta^{k+\frac{2}{3}}-\vtheta^{k}\|,
    \label{eq:thrm4_1_2}
\end{align}
where in the last two inequalities we use the property of the norm.
Before reaching an $\epsilon$-FOSP, Eq. (\ref{eq:thrm4_1_2}) implies that 
\begin{align}
    &-\epsilon\geq \min\limits_{\vtheta\in\mathcal{C}_2}\nabla f(\vtheta^k)^T(\vtheta-\vtheta^{k})\geq-\big(G+\frac{D\sigma_1(\mF^k)}{\eta^k}\big)\|\vtheta^{k+\frac{2}{3}}-\vtheta^{k}\|\nonumber \\ 
    \Rightarrow\quad&\|\vtheta^{k+\frac{2}{3}}-\vtheta^{k}\|\geq\frac{\epsilon}{G+\frac{D\sigma_1(\mF^k)}{\eta^k}}.
    \label{eq:thrm4_1_3}
\end{align}
Based on Eq. (\ref{eq:thrm4_1_1}) and Eq. (\ref{eq:thrm4_1_3}), we have
\begin{align}
    f(\vtheta^{k+\frac{2}{3}})
    &\leq f(\vtheta^{k})-\frac{L}{2}\|\vtheta^{k+\frac{2}{3}}-\vtheta^{k}\|^2-{\nabla f(\vtheta^{k+\frac{2}{3}})^T}(\vtheta^{k+1}-\vtheta^{k+\frac{2}{3}})-\frac{L}{2}{\|\vtheta^{k+1}-\vtheta^{k+\frac{2}{3}}\|^2}\nonumber \\
     &\leq f(\vtheta^{k})-\frac{L\epsilon^2}{2(G+\frac{D\sigma_1(\mF^k)}{\eta^k})^2}-{\nabla f(\vtheta^{k+\frac{2}{3}})^T}(\vtheta^{k+1}-\vtheta^{k+\frac{2}{3}})-\frac{L}{2}{\|\vtheta^{k+1}-\vtheta^{k+\frac{2}{3}}\|^2}.
     \label{eq:thrm4_1_4}
\end{align}
Based on the $L$-Lipschitz continuity of gradients, for the projection to the constraint set $\mathcal{C}_1$ we have
\begin{align}
    f(\vtheta^{k+1})& \leq  f(\vtheta^{k+\frac{2}{3}})+{\nabla f(\vtheta^{k+\frac{2}{3}})^T}(\vtheta^{k+1}-\vtheta^{k+\frac{2}{3}})+\frac{L}{2}{\|\vtheta^{k+1}-\vtheta^{k+\frac{2}{3}}\|^2}.
    \label{eq:thrm4_1_5}
\end{align}
Combining Eq. (\ref{eq:thrm4_1_4}) with Eq. (\ref{eq:thrm4_1_5}), we have
\begin{align}
    f(\vtheta^{k+1}) \leq  f(\vtheta^{k})-\frac{L\epsilon^2}{2(G+\frac{D\sigma_1(\mF^k)}{\eta^k})^2}.
    \label{eq:thrm4_1_6}
\end{align}
Hence it takes $\mathcal{O}(\epsilon^{-2})$ iterations to reach an $\epsilon$-FOSP.

\textbf{\algname\ under the 2-norm projection converges to an $\epsilon$-FOSP.} Based on Lemma \ref{lemma:projecion_appendix} under the 2-norm projection, and setting $\vtheta=\vtheta^k-\eta^k{\mF^k}^{-1}\nabla f(\vtheta^k),$ $\vtheta^*=\vtheta^{k+\frac{2}{3}}$ and $\vtheta'=\vtheta^k,$ we have
\begin{align}
   &(\vtheta^{k}-\vtheta^{k+\frac{2}{3}})^T(\vtheta^k-\eta^k{\mF^k}^{-1}\nabla f(\vtheta^k)-\vtheta^{k+\frac{2}{3}})\leq0\nonumber\\
   \Rightarrow&({\mF^k}^{-1}\nabla f(\vtheta^k))^T(\vtheta^{k+\frac{2}{3}}-\vtheta^{k})\leq - \frac{1}{\eta^k}{(\vtheta^{k+\frac{2}{3}}-\vtheta^{k})^T}(\vtheta^{k+\frac{2}{3}}-\vtheta^{k}).
   \label{eq:appendix_converge_7}
\end{align}
Based on the $L$-Lipschitz continuity of gradients and Eq. (\ref{eq:appendix_converge_7}), we have 
\begin{align}
f(\vtheta^{k+\frac{2}{3}})& \leq  f(\vtheta^{k})+{\nabla f(\vtheta^k)^T}(\vtheta^{k+\frac{2}{3}}-\vtheta^{k})+\frac{L}{2}{\|\vtheta^{k+\frac{2}{3}}-\vtheta^{k}\|^2} \nonumber \\ 
&\leq f(\vtheta^{k}) + ({\mF^k}^{-1}\nabla f(\vtheta^k))^T(\vtheta^{k+\frac{2}{3}}-\vtheta^{k})+Q+\frac{L}{2}{\|\vtheta^{k+\frac{2}{3}}-\vtheta^{k}\|^2}\nonumber \\
&\leq f(\vtheta^{k}) - \frac{1}{\eta^k}{(\vtheta^{k+\frac{2}{3}}-\vtheta^{k})^T}(\vtheta^{k+\frac{2}{3}}-\vtheta^{k})+Q+\frac{L}{2}{\|\vtheta^{k+\frac{2}{3}}-\vtheta^{k}\|^2}\nonumber \\
&= f(\vtheta^{k})-\frac{L}{2}{\|\vtheta^{k+\frac{2}{3}}-\vtheta^{k}\|^2}-{\nabla f(\vtheta^{k+\frac{2}{3}})^T}(\vtheta^{k+1}-\vtheta^{k+\frac{2}{3}})-\frac{L}{2}{\|\vtheta^{k+1}-\vtheta^{k+\frac{2}{3}}\|^2},
\label{eq:appendix_converge_8}
\end{align}
where $Q:=\nabla f(\vtheta^k)^T(\vtheta^{k+\frac{2}{3}}-\vtheta^{k})-({\mF^k}^{-1}\nabla f(\vtheta^k))^T(\vtheta^{k+\frac{2}{3}}-\vtheta^{k})$, which represents the difference between the gradient and the nature gradient, and the equality follows by setting $\delta$ (\ie the size of the trust region) such that
\[
\eta^k=\frac{\|\vtheta^{k+\frac{2}{3}}-\vtheta^{k}\|^2}{L\|\vtheta^{k+\frac{2}{3}}-\vtheta^{k}\|^2+Q+\nabla f(\vtheta^{k+\frac{2}{3}})^T(\vtheta^{k+1}-\vtheta^{k+\frac{2}{3}})+\frac{L}{2}\|\vtheta^{k+1}-\vtheta^{k+\frac{2}{3}}\|^2}.
\]
Again, based on Lemma \ref{lemma:projecion_appendix}, for $\vtheta\in\mathcal{C}_2$ we have 
\begin{align}
    &{(\vtheta^{k}-\eta^k{\mF^k}^{-1}\nabla f(\vtheta^k)-\vtheta^{k+\frac{2}{3}})}(\vtheta-\vtheta^{k+\frac{2}{3}})\leq0 \nonumber \\ 
    \Rightarrow\quad&(-\eta^k{\mF^k}^{-1}\nabla f(\vtheta^k))^T(\vtheta-\vtheta^{k+\frac{2}{3}})\leq-(\vtheta^{k}-\vtheta^{k+\frac{2}{3}})^T(\vtheta-\vtheta^{k+\frac{2}{3}})\nonumber \\ 
    \Rightarrow\quad&\nabla f(\vtheta^k)^T{\mF^k}^{-1}(\vtheta-\vtheta^{k+\frac{2}{3}}) \geq \frac{1}{\eta^k}(\vtheta^{k}-\vtheta^{k+\frac{2}{3}})^T(\vtheta-\vtheta^{k+\frac{2}{3}})\nonumber \\ 
    \Rightarrow\quad& \nabla f(\vtheta^k)^T{\mF^k}^{-1}\vtheta\geq\nabla f(\vtheta^k)^T{\mF^k}^{-1}\vtheta^{k+\frac{2}{3}}+\frac{1}{\eta^k}(\vtheta^k-\vtheta^{k+\frac{2}{3}})^T(\vtheta-\vtheta^{k+\frac{2}{3}})\nonumber \\ 
    \Rightarrow\quad&\nabla f(\vtheta^k)^T{\mF^k}^{-1}(\vtheta-\vtheta^{k})\geq\nabla f(\vtheta^k)^T{\mF^k}^{-1}(\vtheta^{k+\frac{2}{3}}-\vtheta^{k})+\frac{1}{\eta^k}(\vtheta^k-\vtheta^{k+\frac{2}{3}})^T(\vtheta-\vtheta^{k+\frac{2}{3}})\nonumber \\ 
    & \geq -\|\nabla f(\vtheta^k)\|\|{\mF^k}^{-1}\|\|\vtheta^{k+\frac{2}{3}}-\vtheta^{k}\|-\frac{1}{\eta^k}\|\vtheta^{k+\frac{2}{3}}-\vtheta^{k}\|\|\vtheta-\vtheta^{k+\frac{2}{3}}\|\nonumber \\ 
    & \geq -\big(G\sigma_1({\mF^k}^{-1})+\frac{D}{\eta^k}\big)\|\vtheta^{k+\frac{2}{3}}-\vtheta^{k}\|,
    \label{eq:appendix_converge_10}
\end{align}
where in the last two inequalities we use the property of the norm.
Before reaching an $\epsilon$-FOSP, Eq. (\ref{eq:appendix_converge_10}) implies that 
\begin{align}
    &-\epsilon\geq \min\limits_{\vtheta\in\mathcal{C}_2}\nabla f(\vtheta^k)^T{\mF^k}^{-1}(\vtheta-\vtheta^{k})\geq-\big(G\sigma_1({\mF^k}^{-1})+\frac{D}{\eta^k}\big)\|\vtheta^{k+\frac{2}{3}}-\vtheta^{k}\|\nonumber \\ 
    \Rightarrow\quad&\|\vtheta^{k+\frac{2}{3}}-\vtheta^{k}\|\geq\frac{\epsilon}{\big(G\sigma_1({\mF^k}^{-1})+\frac{D}{\eta^k}\big)}.
    \label{eq:appendix_converge_11}
\end{align}
Based on Eq. (\ref{eq:appendix_converge_8}) and Eq. (\ref{eq:appendix_converge_11}), we have
\begin{align}
    f(\vtheta^{k+\frac{2}{3}})
    &\leq f(\vtheta^{k})-\frac{L}{2}\|\vtheta^{k+\frac{2}{3}}-\vtheta^{k}\|^2-{\nabla f(\vtheta^{k+\frac{2}{3}})^T}(\vtheta^{k+1}-\vtheta^{k+\frac{2}{3}})-\frac{L}{2}{\|\vtheta^{k+1}-\vtheta^{k+\frac{2}{3}}\|^2}\nonumber \\
     &\leq f(\vtheta^{k})-\frac{L\epsilon^2}{2({G\sigma_1({\mF^k}^{-1})+\frac{D}{\eta^k}})^2}-{\nabla f(\vtheta^{k+\frac{2}{3}})^T}(\vtheta^{k+1}-\vtheta^{k+\frac{2}{3}})-\frac{L}{2}{\|\vtheta^{k+1}-\vtheta^{k+\frac{2}{3}}\|^2}.
     \label{eq:appendix_converge_12}
\end{align}
Based on the $L$-Lipschitz continuity of gradients, for the projection to the constraint set $\mathcal{C}_1$ we have
\begin{align}
    f(\vtheta^{k+1})& \leq  f(\vtheta^{k+\frac{2}{3}})+{\nabla f(\vtheta^{k+\frac{2}{3}})^T}(\vtheta^{k+1}-\vtheta^{k+\frac{2}{3}})+\frac{L}{2}{\|\vtheta^{k+1}-\vtheta^{k+\frac{2}{3}}\|^2}.
    \label{eq:appendix_converge_13}
\end{align}
Combining Eq. (\ref{eq:appendix_converge_12}) with Eq. (\ref{eq:appendix_converge_13}), we have
\begin{align}
    f(\vtheta^{k+1}) \leq  f(\vtheta^{k})-\frac{L\epsilon^2}{2({G\sigma_1({\mF^k}^{-1})+\frac{D}{\eta^k}})^2}.
    \label{eq:appendix_converge_14}
\end{align}
Hence it takes $\mathcal{O}(\epsilon^{-2})$ iterations to reach an $\epsilon$-FOSP.
\end{proof}

\paragraph{Comments on Assumption 1.3.}
In the paper, we assume that both the diameters of the cost constraint set ($\mathcal{C}_1$) and the region around $\pi_B$ ($\mathcal{C}_2$) are bounded above by $H.$ 
This implies that given a small value for $h_D,$ the convergence speed is determined by how large the constraint set is.
This allows us to do an analysis for the algorithm. 
In practice, we agree that this assumption is too strong and leave it as a future work for improvement.

\paragraph{Interpretation on Theorem \ref{theorem:P2CPO_converge}.}
We now provide a visualization in Fig. \ref{fig:KL_L2_Proj} under two possible projections.
For each projection,
we consider two possible Fisher information matrices.
Please read the caption for more detail.
%
%Theorem \ref{theorem:P2CPO_converge} implies that a smaller $\sigma_1(\mF^k)$ has more improvement of the objective value.
%
%However, the step size $\eta^k$ is also proportional to the KL-divergence between $\vtheta^k$ and $\vtheta^{k+\frac{2}{3}}.$
%
%This implies that the effect of $\sigma_1(\mF^k)$ is canceled out by $\eta^k.$ 
%
In Fig. \ref{fig:KL_L2_Proj}(a) we observe that since the reward improvement and projection steps use the KL-divergence, the resulting two update points with different $\sigma_1(\mF^k)$ are similar.
In addition, under the 2-norm projection, the larger  $\sigma_n(\mF^k)$ is, the greater the decrease in the objective.
%Theorem \ref{theorem:P2CPO_converge} implies that a larger smallest singular value $\sigma_n(\mF^k)$ has more improvement of the objective value.
%
This is because that a large $\sigma_n(\mF^k)$ implies a large curvature of $f$ in all directions. 
Intuitively, this makes the learning algorithm confident about where to update the policy to decrease the objective value greatly.
Geometrically, a large $\sigma_n(\mF^k)$ makes the 2-norm distance between the pre-projection and post-projection points small, leading to a small deviation from the reward improvement direction.
%
%This observation is also supported by the update procedures in Eq. \ref{eq:P2CPO_final}. 
%
%We observe that a large $\sigma_n(\mF^k)$ makes the coefficients of the projection terms small. 
%
%This implies that $\vtheta^{k+1}$ moves toward the direction that can improve the reward most.
%
This is illustrated in Fig. \ref{fig:KL_L2_Proj}(b).
We observe that since $\mF^k$ determines the curvature of $f$ and the 2-norm projection is used, the updated point with a larger $\sigma_n(\mF^k)$ (red dot) achieves more improvement of the objective value.
These observations imply that the spectrum of the Fisher information matrix does not play a major role in \algname\ under the KL-divergence projection, whereas it affects the decrease of objective value in \algname\ under the 2-norm projection.
Hence we choose either KL-divergence or 2-norm projections depending on the tasks to achieve better performance. 
%
%To further illustrate their difference, we compare these two projections  

\begin{figure*}[t]
\vspace{-3mm}
\centering
\subfloat[\algname\ under the KL-divergence projection]{
\includegraphics[width=0.5\linewidth]{figure/KLproj_v2.png}}\hspace{15mm}
\subfloat[\algname\ under the 2-norm projection]{
\includegraphics[width=0.5\linewidth]{figure/L2proj_v2.png}}
\caption{Update procedures for \algname\ under the KL and 2-norm projections with two possible Fisher information matrices.
A lower objective value is achieved at the darker green area.
Red and orange ellipses are $\mF^k$s with two different spectra of singular values.
Red and orange dots are resulting updated points under these two spectra of $\mF^k$s.
\textbf{(a)} A red ellipse has a smaller $\sigma_1(\mF^k)$ and an orange ellipse has a larger $\sigma_1(\mF^k).$ 
Both ellipses have the same $\sigma_n(\mF^k).$ 
The two resulting $\vtheta^{k+\frac{2}{3}}$ are similar.
\textbf{(b)} A red ellipse has a larger $\sigma_n(\mF^k)$ and an orange ellipse has a smaller $\sigma_n(\mF^k).$
Both ellipses have the same $\sigma_1(\mF^k).$ 
$\vtheta^{k+\frac{2}{3}}$ with a larger $\sigma_n(\mF^k)$ (red dot) has greater decrease of the objective value.
}
\label{fig:KL_L2_Proj}
%\end{mdframed}
\end{figure*}

\section{Additional Experiment Results}
\label{sec:appendix_experiment}
\subsection{Implementation Details}
\label{subsec:appendix_details}
\paragraph{Mujoco Task~\cite{achiam2017constrained}.}
In the point circle and ant circle tasks, the reward and cost functions are
\[
R(s) = \frac{\vv^T[-x_2;x_1]}{1+|\|[x_1;x_2]\|-d|},
\]
and
\[
C(s) = \mathbbm{1}[|x_1|>x_\mathrm{lim}],
\]
where $x_1$ and $x_2$ are the coordinates in the plane, $\vv$ is the velocity of the agent, and $d$, $x_\mathrm{lim}$ are environmental parameters that specify the safe area. 
The agent is rewarded for moving fast in a wide circle with radius of $d$, but is constrained to stay within a safe region smaller than the radius of the circle in $x_1$-coordinate $x_\mathrm{lim}\leq d$.
For the point agent, we use $d=5$ and $x_\mathrm{lim}=2.5$; for the ant agent, we use $d=5$ and $x_\mathrm{lim}=1.$
The environment is illustrated in Fig. \ref{fig:circle_env}.

\begin{figure*}[t]
\centering
\includegraphics[scale=0.3]{figure/circle_env.png}
\caption{
The environment of the circle task (adapted from \cite{achiam2017constrained}). The agent receives the maximum reward while staying in the safe area by following the red dashed line path. 
}
\label{fig:circle_env}
\end{figure*}

In the point gather task, the agent receives a reward of $+10$ for gathering green apples, and a cost of $1$ for gathering red apples.
Two green apples and eight red apples are placed in the environment at the beginning.
In the ant gather task, the agent receives a reward of $+10$ for gathering green apples, and a cost of $1$ for gathering red apples.
The agent also gets a reward of $-10$ for falling down to encourage smooth moving. 
Eight green apples and eight red apples are placed in the environment at the beginning.

For the point and ant agents, the state space consists of the positions, orientations, velocities, and the external forces applied to the torso and joint angles. 
The action space is the force applied to joints.

\paragraph{Traffic Management Task~\cite{vinitsky2018benchmarks}.}
In the grid task, the state space, action space, reward function, and cost function are illustrated as follows.
(1) States: Speed, distance to the intersection, and edge number of each vehicle. 
The edges of the grid are uniquely numbered so the travel direction can be inferred. 
For the traffic lights, we return 0 and 1 corresponding to green or red for each light, 
a number between $[0, t_\mathrm{switch}]$ indicating how long until a switch can occur, 
and 0 and 1 indicating if the light is currently yellow. 
Finally, we return the average density and velocity of each edge.

(2) Actions: A list of numbers $a=[-1, 1]^n$ where $n$ is the number of traffic lights. If $a_i>0$ for traffic light $i$ it switches, otherwise no action is taken.

(3) Reward: The objective of the agent is to achieve high speeds. 
The reward function is
\[
R(s) = \frac{\max(v_\mathrm{target}-\|\vv_\mathrm{target}-\vv\|,0)}{v_\mathrm{target}},
\]
where $v_\mathrm{target}$ is an arbitrary large velocity used to encourage high speeds and $\vv\in\R^k$ is the velocities of $k$ vehicles in the network.

(4) Cost: The objective of the agent is to let lights stay red for at most 7 consecutive seconds.
The cost function is 
\[
C(s) = \sum_{i=1}^{n}\mathbbm{1}[t_{i,\mathrm{red}}>7],
\]
where $t_{i,\mathrm{red}}$ is the consecutive time that the light $i$ is in red.

In the bottleneck task, the state space, action space, reward function, and cost function are illustrated as follows.
(1) States: The states include: the mean positions and velocities of human drivers for each lane for each edge segment,
the mean positions and velocities of the autonomous vehicles on each segment, and 
the outflow of the system in vehicles per/hour over the last 5 seconds.
(2) Actions: For a given edge-segment and a given lane, the action shifts the maximum speed
of all the autonomous vehicles in the segment from their current value. 
By shifting the max-speed to higher or lower values, the system indirectly controls the velocity of the autonomous vehicles.
(3) Reward: The objective of the agent is to maximize the outflow of the whole traffic. 
The reward function is
\[
R(s_t) = \sum_{i=t-\frac{5}{\Delta t}}^{i=t}\frac{n_\mathrm{exit}(i)}{\frac{5}{\Delta t\cdot n_\mathrm{lane}\cdot 500}},
\]
where $n_\mathrm{exit}(i)$ is the number of vehicles that exit the system at time-step $i$, and $n_\mathrm{lane}$ is the number of lanes.
(4) Cost: The objective of the agent is to let the velocities of human drivers have lowspeed for no more than 10 seconds.
The cost function is 
\[
C(s) = \sum_{i=1}^{n_\mathrm{human}}\mathbbm{1}[t_{i,\mathrm{low}}>10],
\]
where $n_\mathrm{human}$ is the number of human drivers, and $t_{i,\mathrm{low}}$ is the consecutive time that the velocity of human driver $i$ is less than 5 m/s.
For more information, please refer to \cite{vinitsky2018benchmarks}. 

\paragraph{Car-racing Task.} In the car-racing task, the state space, action space, reward function, and the cost function are illustrated as follows.

(1) States: It is a high-dimensional space where the state is a $96 \times 96 \times 3$ tensor of raw pixels. Each pixel is in the range of $[0,255].$ 

(2) Actions: The agent has 12 actions in total: $a\in\mathcal{A}=\{(a^\mathrm{steer},a^\mathrm{gas},a^\mathrm{brake})|a^\mathrm{steer}\in\{-1,0,1\},a^\mathrm{gas}\in\{0,1\},a^\mathrm{brake}\in\{0,0.2\}\},$ where $a^\mathrm{steer}$ is the steering angle, $a^\mathrm{gas}$ is the amount of gas applied, and $a^\mathrm{brake}$ is the amount of brake applied.

(3) Reward: In each
episode, we randomly generate the track. The episode is terminated if the agent reaches the maximal step or traverse over 95\% of the track.
The track is discretized into 281 tiles.
The agent receives a reward of $\frac{1000}{281}$ for each tile visited. 
To encourage driving efficiency, the agent receives a penalty of $-1$ per-time step. 

(4) Cost: The cost is to constrain the accumulated number of brakes to encourage a smooth ride.

%
%The results, code, and demonstration videos are available at \url{http://www.anonymous}.
%

%
\paragraph{Architectures and Parameters.}
For the gather and circle tasks we test two distinct agents: 
a point-mass ($S \subseteq \R^{9}, A \subseteq \R^{2}$), 
and an ant robot ($S \subseteq \R^{32}, A \subseteq \R^{8}$).
The agent in the grid task is $S \subseteq \R^{156}, A \subseteq \R^{4},$ and the agent in the bottleneck task is $S \subseteq \R^{141}, A \subseteq \R^{20}.$
Finally, the agent in the car-racing task is $S \subseteq \R^{96\times 96\times3}, A \subseteq \R^{3}.$

For the simulations in the gather and circle tasks, we use a neural network with two hidden layers of size (64, 32) to represent Gaussian policies. And we use the KL-divergence projection.
For the simulations in the grid and bottleneck tasks, we use a neural network with two hidden layers of size (16, 16) and (50, 25) to represent Gaussian policies, respectively. And we use the 2-norm projection.
For the simulation in the car-racing task, we use a convolutional neural network with two convolutional operators of size 24 and 12 followed by a dense layer of size (32, 16) to represent a Gaussian policy. And we use the KL-divergence projection.
The choice of the projections depends on the task itself, we report the best performance among two projections.
We use $\mathrm{tanh}$ as an activation function for all the neural network policies.
In the experiments, since the step size is small, we reuse the Fisher information matrix of the reward improvement step in the KL-divergence projection step to reduce the computational cost.
We use GAE-$\lambda$ approach \cite{schulman2015high} to estimate $A^\pi_{R}(s,a),$ $A^\pi_{C}(s,a),$ and $A^\pi_{D}(s).$
For the simulations in the gather, circle, and car-racing tasks, we use neural network baselines with the same architecture and activation functions as the policy networks.
For the simulations in the grid and bottleneck tasks, we use linear baselines.
The hyperparameters of all algorithms and all tasks are in Table \ref{tab:parab}. 

\begin{table*}[t]
\centering
\vspace{0.0in}
\scalebox{0.9}{
\begin{tabular}{cccccccc}
\toprule
Parameter                                      & PC & PG & AC & AG & Gr & BN & CR\\  \hline
\multirow{1}{*}{Reward dis. factor~$\gamma$}      & 0.995 & 0.995 & 0.995 & 0.995 & 0.999 & 0.999 & 0.990 \\
\multirow{1}{*}{Constraint cost dis. factor~$\gamma_{C}$}      & 1.0  & 1.0  & 1.0  & 1.0  & 1.0  & 1.0  & 1.0 \\
\multirow{1}{*}{Divergence cost dis. factor~$\gamma_{D}$}      & 1.0 & 1.0 & 1.0 & 1.0 & 1.0  & 1.0 & 1.0 \\
\multirow{1}{*}{step size~$\delta$}             & $10^{-4}$ & $10^{-4}$ & $10^{-4}$ & $10^{-4}$ & $10^{-4}$ & $10^{-4}$ & $5\times10^{-4}$ \\
\multirow{1}{*}{$\lambda^\mathrm{GAE}_{R}$}    & 0.95 & 0.95 & 0.95 & 0.95 & 0.97 & 0.97 & 0.95 \\
\multirow{1}{*}{$\lambda^\mathrm{GAE}_{C}$}    & 1.0 & 1.0 & 0.5 & 0.5 & 0.5 & 1.0 & 1.0 \\
\multirow{1}{*}{$\lambda^\mathrm{GAE}_{D}$}    & 0.95 & 0.95 & 0.95 & 0.95 & 0.90 &0.90 & 0.95 \\
\multirow{1}{*}{Batch size}                    & 50,000 & 50,000 & 100,000 & 100,000 & 10,000 & 25,000 & 10,000 \\
\multirow{1}{*}{Rollout length}                & 50 & 15 & 500 & 500 & 400 & 500 & 1000 \\
\multirow{1}{*}{Constraint cost threshold~$h_C$} & 5 & 0.5 & 5 & 0.2 & 0 & 0 & 5 \\
\multirow{1}{*}{Divergence cost threshold~$h_D^0$} & 5 & 3 & 5 & 3 & 10 & 10 & 5 \\
\multirow{1}{*}{Number of policy updates} & 1,000 & 1,200 & 2,500 & 1,500 & 200 & 300 & 600 \\
\bottomrule
\end{tabular}}
\caption{\label{tab:parab}Parameters used in all tasks. (PC: point circle, PG: point gather, AC: ant circle, AG: ant gather, Gr: grid, BN: bottleneck, and CR: car-racing tasks)}
\end{table*}

We conduct the experiments on three separate machines: machine A has an Intel Core i7-4770HQ CPU, machine B has an Intel Core i7-6850K CPU, and machine C has an Intel Xeon X5675 CPU. We report real-time (\ie wall-clock time) in seconds for one policy update for all tested algorithms and tasks in Table \ref{tab:time}.
We observe that \algname\ has the same computational time as the other baselines.

\begin{table*}[t]
\centering
\scalebox{0.8}{
\begin{tabular}{l*{12}{c}r} 
\toprule
&\multicolumn{2}{c}{PCPO}&\multicolumn{2}{c}{\algname\ (Ours)}&\multicolumn{2}{c}{f-PCPO}&\multicolumn{2}{c}{f-CPO}&\multicolumn{2}{c}{d-PCPO}&\multicolumn{2}{c}{d-CPO}\\

\cmidrule(lr){2-3} \cmidrule(lr){4-5}\cmidrule(lr){6-7}\cmidrule(lr){8-9}\cmidrule(lr){10-11}\cmidrule(lr){12-13}

& M/C & Time & M/C & Time & M/C & Time & M/C & Time & M/C & Time & M/C & Time \\ \hline
PG  & B & 22.14 & B & 25.2 & B & 31.9 & B & 25.5   & B & 32.8 & B &32.6\\
PC  & B & 35.1 & B & 51.2 & B & 48.4 & B & 49.4  & B & 55.5 & B & 55.9\\
AG  & B & 386.9 & B & 110.5 & C & 268.6 & C & 235.1  & B & 138.2 & B & 187.5 \\
AC  & B & 148.9 & B & 94.0 & C & 222.6 & C & 214.6   & B & 177.4 & B & 151.2\\
Gr  & A & 105.3 & A & 91.4 & A & 88.2 & A & 58.7  & A & 116.8 & A & 115.3 \\
BN  & A & 257.7 & A & 181.1 & A & 162.9 & A & 161.6   & A & 259.3 & A & 275.6\\
CR  & C & 993.5 & C & 971.6 & C & 1078.3 & C & 940.1  & C & 1000.4 & C & 981.0 \\
\bottomrule
\end{tabular}}
\caption{\label{tab:time}Real-time in seconds for one policy update for all tested algorithms and tasks. (PC: point circle, PG: point gather, AC: ant circle, AG: ant gather, Gr: grid, BN: bottleneck, and CR: car-racing tasks)}
\end{table*}

For the most intensive task, \ie the car-racing task, the memory usage is 6.28GB. 
The experiments are implemented in rllab~\cite{duan2016benchmarking}, 
a tool for developing RL algorithms. 
We provide the link to the code: \url{https://sites.google.com/view/spacealgo}.

\paragraph{Comments on the rationale behind when to increase $h_D$.}
The update method of $h_D$ is empirically designed to ensure that the value of the cost does not increase (\ie $J_C({\pi^k})\leq J_C(\pi^{k-1})$) and the reward keeps improving (\ie $J_R(\pi^k)\geq  J_R(\pi^{k-1})$) after learning from $\pi_B$.
Lemma \ref{theorem:h_D} theoretically ensures $h_D$ is large enough to guarantee feasibility and exploration of the agent.

\paragraph{Implementation of Updating $h_D^k$.}
Lemma \ref{theorem:h_D} shows that $h^{k+1}_D$ should be increased at least by $\mathcal{O}\big((J_{C}(\pi^k)-h_C)^2\big)+h_D^k$ if $J_C(\pi^k)>J_C(\pi^{k-1})$ or $J_R(\pi^k)<J_R(\pi^{k-1})$ at step $k$. 
We now provide the practical implementation.
For each policy update we check the above conditions.
If one of the conditions satisfies, we increase $h_D^{k+1}$ by setting the constant to $10$, \ie $10\cdot(J_{C}(\pi^k)-h_C)^2+h_D^k.$
In practice, we find that the performance of \algname\ is not affected by the selection of the constant.
Note that we could still compute the exact value of $h_D^{k+1}$ as shown in the proof of Lemma \ref{theorem:h_D}.
However, this incurs the computational cost.

\paragraph{Comments on learning from multiple baseline policies $\pi_B$.}
In our setting, we use one $\pi_B$. 
This allows us to do theoretical analysis.
One possible idea for learning from multiple $\pi_B$ is to compute the distance to each $\pi_B$.
Then, select the one with the minimum distance to do the update.
This ensures that the update for the reward in the first step is less affected by $\pi_B.$
And the analysis we did can be extended.
We leave it as future work for developing this.

\paragraph{Comments on refining the PCPO agent's policy~\cite{yang2020projection} directly.}
Fine-tuning the pre-trained policy directly might result in lower reward and cost violations.
This is because that the pre-trained policy has a low entropy and it does not explore.
We empirically observe that the agent pre-trained with the baseline policy yields less reward in the new task (\ie different cost constraint thresholds $h_C$) as illustrated in Section \ref{additional_Experiment}.
In contrast, the \algname\ agent simultaneously learns from the baseline policy while ensuring the policy entropy is high enough to explore the environment.

\parab{Comments on the feasibility of getting safe baseline policies.}
In many real-world applications such as drones, we can obtain baseline policies modeled from the first principle physics, or pre-train baseline policies in the constrained and safe environment, or use rule-based baseline policies. Importantly, we do not assume the baseline has to be a ``safe policy'' -- it can be a heuristic that ignores safety constraints. This is one of the main motivations for our algorithm: to utilize priors from the baseline which may be unsafe, but guarantee the safety of the newly learned algorithm according to the provided constraints.

\paragraph{Instructions for Reproducibility.}
We now provide the instructions for reproducing the results.
First install the libraries for python3 such as numpy, scipy.
To run the Mujoco experiments, get the licence from \url{https://www.roboti.us/license.html}.
To run the traffic management experiments, install FLOW simulator from \url{https://flow.readthedocs.io/en/latest/}.
To run the car-racing experiments, install OpenAI Gym from \url{https://github.com/openai/gym}.
Our implementation is based on the environment from \cite{achiam2017constrained}, please download the code from \url{https://github.com/jachiam/cpo}. 
The code is based on rllab \cite{duan2016benchmarking}, install the relevant packages such as theano (\url{http://deeplearning.net/software/theano/}).
Then, download \algname\ code from \url{https://sites.google.com/view/spaceneurips} and place the codes on the designated folder instructed by Readme.txt on the main folder.
Finally, go to the example folder and execute the code using python command.

\begin{figure*}[t]
\vspace{-3mm}
\centering
\subfloat[Bottleneck\label{subfig:bn}]{\begin{tabular}[b]{@{}c@{}}%
\includegraphics[width=0.33\linewidth]{figure/exp_2/RewardvsCost_bn_overallPerformance_v2.png}%
\end{tabular}}%
\subfloat[Car-racing\label{subfig:cr}]{\begin{tabular}[b]{@{}c@{}}%
\includegraphics[width=0.33\linewidth]{figure/exp_2/RewardvsCost_cr_overallPerformance_v2.png}%
\end{tabular}}%
\subfloat[Grid\label{subfig:grid}]{\begin{tabular}[b]{@{}c@{}}%
\includegraphics[width=0.33\linewidth]{figure/exp_2/RewardvsCost_gr_overallPerformance_v2.png}%
\end{tabular}}%
\iffalse
\subfloat[Point gather\label{subfig:pg}]{\begin{tabular}[b]{@{}c@{}}%
\includegraphics[width=0.33\linewidth]{figure/exp_2/RewardvsCost_pg_SafevsAggressive.png}%
\\
\includegraphics[width=0.33\linewidth]{figure/exp_2/NumDemo_pg_SafevsAggressive.png}%
\end{tabular}}%
\subfloat[Ant circle\label{subfig:ac}]{\begin{tabular}[b]{@{}c@{}}%
\includegraphics[width=0.33\linewidth]{figure/exp_2/RewardvsCost_ac_Dynamic_hp_and_fixed_hp.png}%
\\
\includegraphics[width=0.33\linewidth]{figure/exp_2/NumDemo_ac_Dynamic_hp_and_fixed_hp.png}%
\end{tabular}}%
\fi
\vspace{+1mm}

\includegraphics[width=0.9\linewidth]{figure/exp_2/legend_cum.png}
\vspace{-2mm}

\caption{
The discounted reward vs. the cumulative undiscounted constraint cost
over policy updates for the tested algorithms and tasks.
The solid line is the mean over 5 runs.
\algname\ achieves the same reward performance with fewer cost constraint violations in all cases.
%The baseline policies in the gird and bottleneck tasks are $\pi_B^\mathrm{same},$
%
%and the baseline policy in the car-racing task is $\pi_B^\mathrm{human}.$
%
%The values of the discounted reward, the undiscounted cost constraint value, and the undiscounted prior constraint value under two different priors over policy updates for the tested algorithms and task pairs. 
%
%The solid line is the mean and the shaded area is the standard deviation over five runs. 
%
%The dashed lines in the reward plot are the rewards of $\pi_B^\mathrm{cost}$ (lower) and $\pi_B^\mathrm{reward}$ (upper).
%
%The dashed lines in the cost constraint plot are the cost constraint value of the $\pi_B^\mathrm{cost}$ (lower) and $\pi_B^\mathrm{reward}$ (upper).
%
%The middle dashed line in the cost constraint plot is the cost constraint threshold $h_C$ of the agent.
%
%We observe that \algname\ with a safe prior $\pi^\mathrm{cost}_B$ achieves better reward performance compared to the one with an aggressive prior $\pi^\mathrm{reward}_B.$
%
(Best viewed in color.)
}
\label{fig:reward_vs_cost}
\vspace{-3mm}
%\end{mdframed}
\end{figure*}

\subsection{Experiment Results}
\label{additional_Experiment}

\paragraph{Baseline policies.}
We pre-train the baseline policies using a safe RL algorithm. 
Here we also consider three types of baseline policies:
\textbf{(1)} \textit{suboptimal} $\pi_B^\mathrm{cost}$ with $J_C(\pi_B^\mathrm{cost})\approx0,$
\textbf{(2)} \textit{suboptimal} $\pi_B^\mathrm{reward}$ with $J_C(\pi_B^\mathrm{reward})>h_C,$ 
and 
\textbf{(3)} $\pi_B^\mathrm{near}$ with $J_C(\pi_B^\mathrm{near})\approx h_C$
Note that these $\pi_B$ have different degrees of constraint satisfaction.

\paragraph{The Discounted Reward vs. the Cumulative Undiscounted Constraint Cost (see Fig.~\ref{fig:reward_vs_cost}).}
To show that \algname\ achieves higher reward under the same cost constraint violations (\ie learning a constraint-satisfying policy without violating the cost constraint a lot), we examine the discounted reward versus the \textit{cumulative} undiscounted constraint cost.
The learning curves of the discounted reward versus the cumulative undiscounted constraint cost are shown for all tested algorithms and tasks in Fig. \ref{fig:reward_vs_cost}.
We observe that in these tasks under the same value of the reward, \algname\ outperforms the baselines significantly with fewer cost constraint violations. 
For example, in the car-racing task \algname\ achieves 3 times fewer cost constraint violations at the reward value of 40 compared to the best baseline -- PCPO.
This implies that \algname\ effectively leverages the baseline policy while ensuring the constraint satisfaction.
In contrast, without the supervision of the baseline policy, PCPO requires much more constraint violations to achieve the same reward performance as \algname.
In addition, although the fixed-point and the dynamic-point approaches use the supervision of the baseline policy, the lack of the projection step makes them less efficient in learning a constraint-satisfying policy.

\begin{figure*}[t]
\vspace{-3mm}
\centering
\subfloat[Point gather\label{subfig:grid}]{\begin{tabular}[b]{@{}c@{}}%
\includegraphics[width=0.33\linewidth]{figure/exp_2/NumCost_pg_overallPerformance_v2.png}%
\includegraphics[width=0.33\linewidth]{figure/exp_2/Reward_pg_overallPerformance_v2.png}%
\includegraphics[width=0.33\linewidth]{figure/exp_2/NumDemo_pg_overallPerformance_v2.png}%
\end{tabular}}%

\subfloat[Point circle\label{subfig:grid}]{\begin{tabular}[b]{@{}c@{}}%
\includegraphics[width=0.33\linewidth]{figure/exp_2/NumCost_pc_overallPerformance_v2.png}%
\includegraphics[width=0.33\linewidth]{figure/exp_2/Reward_pc_overallPerformance_v2.png}%
\includegraphics[width=0.33\linewidth]{figure/exp_2/NumDemo_pc_overallPerformance_v2.png}%
\end{tabular}}%

\subfloat[Ant gather\label{subfig:bn}]{\begin{tabular}[b]{@{}c@{}}%
\includegraphics[width=0.33\linewidth]{figure/exp_2/NumCost_ag_overallPerformance_v2.png}%
\includegraphics[width=0.33\linewidth]{figure/exp_2/Reward_ag_overallPerformance_v2.png}%
\includegraphics[width=0.33\linewidth]{figure/exp_2/NumDemo_ag_overallPerformance_v2.png}%
\end{tabular}}%

\subfloat[Ant circle 
%(Note that the y-axis of the reward and cost constraint plots is in log-scale. The reward values of two priors are roughly the same but with very different cost values.)
\label{subfig:cr}]{\begin{tabular}[b]{@{}c@{}}%
\includegraphics[width=0.33\linewidth]{figure/exp_2/NumCost_ac_overallPerformance_v2.png}%
\includegraphics[width=0.33\linewidth]{figure/exp_2/Reward_ac_overallPerformance_v2.png}%
\includegraphics[width=0.33\linewidth]{figure/exp_2/NumDemo_ac_overallPerformance_v2.png}%
\end{tabular}}%

\vspace{+1mm}

\includegraphics[width=0.9\linewidth]{figure/exp_2/legend_2_H.png}
\vspace{-2mm}

\caption{
The undiscounted constraint cost,
the discounted reward, and
the undiscounted divergence cost
over policy updates for the tested algorithms and tasks.
The solid line is the mean and the shaded area is the standard deviation over 5 runs.
\algname\ ensures cost constraint satisfaction guided by the baseline policy which need not satisfy the cost constraint.
%
%The baseline policies in the gird and bottleneck tasks are $\pi_B^\mathrm{same},$
%
%and the baseline policy in the car-racing task is $\pi_B^\mathrm{human}.$
%
%The values of the discounted reward, the undiscounted cost constraint value, and the undiscounted prior constraint value under two different priors over policy updates for the tested algorithms and task pairs. 
%
%The solid line is the mean and the shaded area is the standard deviation over five runs. 
%
%The dashed lines in the reward plot are the rewards of $\pi_B^\mathrm{cost}$ (lower) and $\pi_B^\mathrm{reward}$ (upper).
%
%The dashed lines in the cost constraint plot are the cost constraint value of the $\pi_B^\mathrm{cost}$ (lower) and $\pi_B^\mathrm{reward}$ (upper).
%
%The middle dashed line in the cost constraint plot is the cost constraint threshold $h_C$ of the agent.
%
%We observe that \algname\ with a safe prior $\pi^\mathrm{cost}_B$ achieves better reward performance compared to the one with an aggressive prior $\pi^\mathrm{reward}_B.$
%
(Best viewed in color.)
}
\label{fig:appendix_safeAggressivePriors}
\vspace{-5mm}
%\end{mdframed}
\end{figure*}

\paragraph{Comparison of Baseline Policies (see Fig.~\ref{fig:appendix_safeAggressivePriors}).}
To examine whether \algname\ can safely learn from the baseline policy which need not satisfy the cost constraint,
we consider two baseline policies: $\pi^\mathrm{cost}_B$ and $\pi^\mathrm{reward}_B.$
The learning curves of the undiscounted constraint cost, the discounted reward, and the undiscounted divergence cost with two possible baselines over policy updates are shown for all tested algorithms and tasks in Fig. \ref{fig:appendix_safeAggressivePriors}.
We observe that in the point gather and point circle tasks, the initial values of the cost are larger than $h_C$ (\ie $J_C(\pi^0)>h_C$).
%
%This implies that the initial policies are outside the cost constraint sets.
%
Using $\pi^\mathrm{cost}_B$ allows the learning algorithm to quickly satisfy the cost without doing the extensive projection onto the cost constraint set.
For example, in the point circle task we observe that learning guided by $\pi^\mathrm{cost}_B$ quickly satisfies the cost constraint.
In addition, we observe that in the ant gather and ant circle tasks, the initial values of the cost are smaller than $h_C$ (\ie $J_C(\pi^0)<h_C$).
%
%This implies that the initial policies are inside the cost constraint sets.
%
Intuitively, we would expect that using $\pi^\mathrm{reward}_B$ allows the agent to quickly improve the reward since the agent already satisfies the cost constraint in the beginning.
In the ant gather task we observe that \algname\ guided by $\pi^\mathrm{reward}_B$ does improve the reward more quickly at around 200 iteration.
However, we observe that the agent guided by the both baseline policies achieve the same final reward performance in the ant gather and ant circle tasks.
The reason is that using dynamic $h_D$ allows the agent to stay away from the baseline policy. 
This makes the baseline policy less influential in the end. 
As a result, the reward improvement mostly comes from the reward improvement step of \algname\ if the agent starts in the interior of the cost constraint set (\ie $J_C(\pi^0)\leq h_C$).

\paragraph{Fixed $h_D$ (see Fig. \ref{fig:appendix_priorConstraintThreshold}).} 
To understand the effect of using dynamic $h_D^k$ when learning from a sub-optimal baseline policy,
we compare the performance of \algname\ with and without adjusting $h_D.$ 
The learning curves of the undiscounted constraint cost, the discounted reward, and the undiscounted divergence cost over policy updates are shown for all tested algorithms and tasks in Fig. \ref{fig:appendix_priorConstraintThreshold}.
We observe that \algname\ with fixed $h_D$ converges to less reward.
For example, in the ant circle task \algname\ with the dynamic $h_D$ achieves 2.3 times more reward.
The value of the divergence cost in the ant circle task shows that staying away from the baseline policy achieves more reward.
This implies that the baseline policy in the ant circle task is highly sub-optimal to the agent.
In addition, we observe that in some tasks the dynamic $h_D$ does not have much effect on the reward performance.
For example, in the point gather task \algname\ achieves the same reward performance. 
The values of the divergence cost in the point gather task decrease throughout the training.
These observations imply that the update scheme of $h_D$ is critical for some tasks.
%
%In contrast, the fixed-point and dynamic-point approaches do not provide this kind of freedom, and hence converge to less reward.

\begin{figure*}[t]
\vspace{-3mm}
\centering
\subfloat[Point gather\label{subfig:cr}]{\begin{tabular}[b]{@{}c@{}}%
\vspace{-3mm}
\includegraphics[width=0.33\linewidth]{figure/exp_2/NumCost_pg_overallPerformance_v2_fixed_dynamic_hp.png}%
\includegraphics[width=0.33\linewidth]{figure/exp_2/Reward_pg_overallPerformance_v2_fixed_dynamic_hp.png}%
\includegraphics[width=0.33\linewidth]{figure/exp_2/NumDemo_pg_overallPerformance_v2_fixed_dynamic_hp.png}%
\end{tabular}}%
\vspace{-3mm}

\subfloat[Point circle\label{subfig:cr}]{\begin{tabular}[b]{@{}c@{}}%
\vspace{-3mm}
\includegraphics[width=0.33\linewidth]{figure/exp_2/NumCost_pc_overallPerformance_v2_fixed_dynamic_hp.png}%
\includegraphics[width=0.33\linewidth]{figure/exp_2/Reward_pc_overallPerformance_v2_fixed_dynamic_hp.png}%
\includegraphics[width=0.33\linewidth]{figure/exp_2/NumDemo_pc_overallPerformance_v2_fixed_dynamic_hp.png}%
\end{tabular}}%
\vspace{-3mm}

\subfloat[Ant gather\label{subfig:cr}]{\begin{tabular}[b]{@{}c@{}}%
\vspace{-3mm}
\includegraphics[width=0.33\linewidth]{figure/exp_2/NumCost_ag_overallPerformance_v2_fixed_dynamic_hp.png}%
\includegraphics[width=0.33\linewidth]{figure/exp_2/Reward_ag_overallPerformance_v2_fixed_dynamic_hp.png}%
\includegraphics[width=0.33\linewidth]{figure/exp_2/NumDemo_ag_overallPerformance_v2_fixed_dynamic_hp.png}%
\end{tabular}}%
\vspace{-3mm}

\subfloat[Ant circle\label{subfig:cr}]{
\begin{tabular}[b]{@{}c@{}}%
\vspace{-3mm}
\includegraphics[width=0.33\linewidth]{figure/exp_2/NumCost_ac_overallPerformance_v2_fixed_dynamic_hp.png}%
\includegraphics[width=0.33\linewidth]{figure/exp_2/Reward_ac_overallPerformance_v2_fixed_dynamic_hp.png}%
\includegraphics[width=0.33\linewidth]{figure/exp_2/NumDemo_ac_overallPerformance_v2_fixed_dynamic_hp.png}%
\end{tabular}}%
\vspace{-3mm}

\subfloat[Car-racing\label{subfig:cr}]{\begin{tabular}[b]{@{}c@{}}%
\vspace{-3mm}
\includegraphics[width=0.33\linewidth]{figure/exp_2/NumCost_cr_overallPerformance_v2_fixed_dynamic_hp.png}%
\includegraphics[width=0.33\linewidth]{figure/exp_2/Reward_cr_overallPerformance_v2_fixed_dynamic_hp.png}%
\includegraphics[width=0.33\linewidth]{figure/exp_2/NumDemo_cr_overallPerformance_v2_fixed_dynamic_hp.png}%
\end{tabular}}%

\vspace{+1mm}

\includegraphics[width=0.55\linewidth]{figure/exp_2/legend_fixhD.png}
\vspace{-2mm}

\caption{
%The values of the discounted reward, the undiscounted constraint value, and the undiscounted prior constraint value over policy updates with and without the relaxation step for the tested algorithms and task pairs.
The undiscounted constraint cost,
the discounted reward, and
the undiscounted divergence cost
over policy updates for the tested algorithms and tasks.
The solid line is the mean and the shaded area is the standard deviation over 5 runs.
\algname\ with the dynamic $h_D$ achieves higher reward.
(Best viewed in color.)
}
\label{fig:appendix_priorConstraintThreshold}
\vspace{-3mm}
%\end{mdframed}
\end{figure*}

\paragraph{Comparison of \algname\ vs. d-CPO, d-PCPO and the Pre-training Approach (see Fig.~\ref{fig:appendix_pretrainingPrior}).} 
To show that \algname\ is effective in using the supervision of the baseline policy, we compare the performance of \algname\ to the dynamic-point and the pre-training approaches.
In the pre-training approach, the agent first performs the trust region update with the objective function being the divergence cost.
Once the agent has the same reward performance as the baseline policy (\ie $J_R(\pi^k)\approx J_R(\pi_B)$ for some $k$), the agent performs the trust region update with the objective function being the reward function.
The learning curves of the undiscounted constraint cost, the discounted reward, and the undiscounted divergence cost over policy updates are shown for all tested algorithms and tasks in Fig. \ref{fig:appendix_pretrainingPrior}.
We observe that \algname\ achieves better reward performance compared to the pre-training approach in all tasks.
For example, in the point circle, ant gather and ant circle tasks the pre-training approach seldom improves the reward but all satisfies the cost constraint.
This implies that the baseline policies in these tasks are highly sub-optimal in terms of reward performance.
In contrast, \algname\ prevents the agent from converging to a poor policy.
In addition, we observe that in the point gather task the pre-training approach achieves the same reward performance as the baseline policy, whereas \algname\ has a better reward performance compared to the baseline policy.
The pre-training approach does not keep improving the reward after learning from the baseline policy.
This is because that after pre-training with the baseline policy, the entropy of the learned policy is small.
This prevents the agent from trying new actions which may lead to better reward performance.
This implies that pre-training approach may hinder the exploration of the learning agent on the new environment.
Furthermore, in the car-racing task we observe that using pre-training approach achieves the same reward performance as \algname\ but improves reward slowly, and the pre-training approach has more cost constraint violations than \algname.
This implies that jointly using reinforcement learning and the supervision of the baseline policy achieve better reward and cost performance.
For d-CPO and d-PCPO, in the point and ant tasks we observe that both approaches have comparable or silently better reward and cost performance compared to \algname.
However, in the car-racing task we observe that d-CPO cannot improve the reward due to a slow update procedure for satisfying the cost constraint, whereas d-PCPO has a better reward performance.
These observations imply that the projection steps in \algname\ allow the learning agent to effectively and robustly learn from the baseline policy.

\begin{figure*}[t]
\vspace{-3mm}
\centering
\subfloat[Point gather\label{subfig:cr}]{\begin{tabular}[b]{@{}c@{}}%
\vspace{-3mm}
\includegraphics[width=0.33\linewidth]{figure/exp_2/NumCost_pg_overallPerformance_v2_d_type_algo.png}%
\includegraphics[width=0.33\linewidth]{figure/exp_2/Reward_pg_overallPerformance_v2_d_type_algo.png}%
\includegraphics[width=0.33\linewidth]{figure/exp_2/NumDemo_pg_overallPerformance_v2_d_type_algo.png}%
\end{tabular}}%
\vspace{-3mm}

\subfloat[Point circle\label{subfig:cr}]{\begin{tabular}[b]{@{}c@{}}%
\vspace{-3mm}
\includegraphics[width=0.33\linewidth]{figure/exp_2/NumCost_pc_overallPerformance_v2_d_type_algo.png}%
\includegraphics[width=0.33\linewidth]{figure/exp_2/Reward_pc_overallPerformance_v2_d_type_algo.png}%
\includegraphics[width=0.33\linewidth]{figure/exp_2/NumDemo_pc_overallPerformance_v2_d_type_algo.png}%
\end{tabular}}%
\vspace{-3mm}

\subfloat[Ant gather\label{subfig:cr}]{\begin{tabular}[b]{@{}c@{}}%
\vspace{-3mm}
\includegraphics[width=0.33\linewidth]{figure/exp_2/NumCost_ag_overallPerformance_v2_d_type_algo.png}%
\includegraphics[width=0.33\linewidth]{figure/exp_2/Reward_ag_overallPerformance_v2_d_type_algo.png}%
\includegraphics[width=0.33\linewidth]{figure/exp_2/NumDemo_ag_overallPerformance_v2_d_type_algo.png}%
\end{tabular}}%
\vspace{-3mm}

\subfloat[Ant circle\label{subfig:cr}]{\begin{tabular}[b]{@{}c@{}}%
\vspace{-3mm}
\includegraphics[width=0.33\linewidth]{figure/exp_2/NumCost_ac_overallPerformance_v2_d_type_algo.png}%
\includegraphics[width=0.33\linewidth]{figure/exp_2/Reward_ac_overallPerformance_v2_d_type_algo.png}%
\includegraphics[width=0.33\linewidth]{figure/exp_2/NumDemo_ac_overallPerformance_v2_d_type_algo.png}%
\end{tabular}}%
\vspace{-3mm}

\subfloat[Car-racing\label{subfig:cr}]{\begin{tabular}[b]{@{}c@{}}%
\vspace{-3mm}
\includegraphics[width=0.33\linewidth]{figure/exp_2/NumCost_cr_annealing_pretraining.png}%
\includegraphics[width=0.33\linewidth]{figure/exp_2/Reward_cr_annealing_pretraining.png}%
\includegraphics[width=0.33\linewidth]{figure/exp_2/NumDemo_cr_annealing_pretraining.png}%
\end{tabular}}%

\vspace{+1mm}

\includegraphics[width=0.75\linewidth]{figure/exp_2/legend_pretrain.png}
\vspace{-2mm}

\caption{
The undiscounted constraint cost,
the discounted reward, and
the undiscounted divergence cost
over policy updates for the tested algorithms and tasks.
The solid line is the mean and the shaded area is the standard deviation over 5 runs.
\algname\ outperforms d-CPO, d-PCPO and the pre-training approach in terms of the efficiency of the reward improvement and cost constraint satisfaction. 
(Best viewed in color.)
}
\label{fig:appendix_pretrainingPrior}
\vspace{-3mm}
%\end{mdframed}
\end{figure*}

\paragraph{Comparison of \algname\ under the KL-divergence and the 2-norm Projections (see Fig.~\ref{fig:appendix_KLvsL2projections}).} 
Theorem \ref{theorem:P2CPO_converge} shows that under the KL-divergence and 2-norm projections, \algname\ converges to different stationary points.
To demonstrate the difference between these two projections, Fig.~\ref{fig:appendix_KLvsL2projections} shows the learning curves of the undiscounted constraint cost, the discounted reward, and the undiscounted divergence cost over policy updates for all tested algorithms and tasks.
In the Mujoco tasks, we observe that \algname\ under the KL-divergence projection achieves higher reward.
For instance, in the point gather task the final reward is 25\% higher under the same cost constraint satisfaction.  
In contrast, in the traffic management tasks, we observe that \algname\ under the 2-norm projection achieves better cost constraint satisfaction.
For instance, in the grid task \algname\ under the 2-norm projection achieves a lower reward but more cost constraint satisfaction. In addition, in the bottleneck task \algname\ under the 2-norm projection achieves more reward and cost constraint satisfaction.
These observations imply that \algname\ converges to different stationary points under two possible projections depending on tasks.

\begin{figure*}[t]
\vspace{-3mm}
\centering

\subfloat[Point gather\label{subfig:ac}]{\begin{tabular}[b]{@{}c@{}}%
\includegraphics[width=0.33\linewidth]{figure/exp_2/NumCost_pg_overallPerformance_v2_KLvsL2projections.png}%
\includegraphics[width=0.33\linewidth]{figure/exp_2/Reward_pg_overallPerformance_v2_KLvsL2projections.png}%
\includegraphics[width=0.33\linewidth]{figure/exp_2/NumDemo_pg_overallPerformance_v2_KLvsL2projections.png}%
\end{tabular}}%

\subfloat[Point circle\label{subfig:ac}]{\begin{tabular}[b]{@{}c@{}}%
\includegraphics[width=0.33\linewidth]{figure/exp_2/NumCost_pc_overallPerformance_v2_KLvsL2projections.png}%
\includegraphics[width=0.33\linewidth]{figure/exp_2/Reward_pc_overallPerformance_v2_KLvsL2projections.png}%
\includegraphics[width=0.33\linewidth]{figure/exp_2/NumDemo_pc_overallPerformance_v2_KLvsL2projections.png}%
\end{tabular}}%

\subfloat[Grid\label{subfig:ac}]{\begin{tabular}[b]{@{}c@{}}%
\includegraphics[width=0.33\linewidth]{figure/exp_2/NumCost_gr_overallPerformance_v2_KLvsL2projections.png}%
\includegraphics[width=0.33\linewidth]{figure/exp_2/Reward_gr_overallPerformance_v2_KLvsL2projections.png}%
\includegraphics[width=0.33\linewidth]{figure/exp_2/NumDemo_gr_overallPerformance_v2_KLvsL2projections.png}%
\end{tabular}}%

\subfloat[Bottleneck\label{subfig:cr}]{\begin{tabular}[b]{@{}c@{}}%
\includegraphics[width=0.33\linewidth]{figure/exp_2/NumCost_bn_overallPerformance_v2_KLvsL2projections.png}%
\includegraphics[width=0.33\linewidth]{figure/exp_2/Reward_bn_overallPerformance_v2_KLvsL2projections.png}%
\includegraphics[width=0.33\linewidth]{figure/exp_2/NumDemo_bn_overallPerformance_v2_KLvsL2projections.png}%
\end{tabular}}%

\vspace{+1mm}

\includegraphics[width=0.7\linewidth]{figure/exp_2/legend_proj.png}
\vspace{-2mm}

\caption{The undiscounted constraint cost,
the discounted reward, and
the undiscounted divergence cost
over policy updates for the tested algorithms and tasks.
The solid line is the mean and the shaded area is the standard deviation over 5 runs.
\algname\ converges to differently stationary points under two possible projections.
(Best viewed in color.)
}
\label{fig:appendix_KLvsL2projections}
\vspace{-3mm}
%\end{mdframed}
\end{figure*}

\paragraph{Initial $h^0_D$ (see Fig. \ref{fig:appendix_initialPriorConstraintThreshold}).} 
%
%\algname\ constructs the prior constraint set to safely learn from the prior.
%
%One question is that how we can select an appropriate initial value of $h_D^0.$
%
To understand the effect of the initial value of $h^0_D,$ we test \algname\ with three different initial values: $h_D^0=1, h_D^0=5,$ and $h_D^0=25$ in the ant circle and car-racing tasks. 
The learning curves of the undiscounted constraint cost, the discounted reward, and the undiscounted divergence cost over policy updates are shown for all tested algorithms and tasks in Fig. \ref{fig:appendix_initialPriorConstraintThreshold}.
In both tasks, we observe that the initial value of $h_D^0$ does not affect the reward and the cost performance significantly (\ie the mean of learning curves lies in roughly the same standard deviation over the initialization).
In addition, the value of the divergence cost over three $h_D^0$ are similar throughout the training.
These observations imply that the update scheme of $h_D^k$ in \algname\ is robust to the choice of the initial value of $h_D^0.$
However, in the car-racing task we observe that the learning curves of using a smaller $h^0_D$ tend to have higher variances.
For example, the standard deviation of $h_D^0=1$ in the reward plot is 6 times larger than the one with $h_D^0=25.$
This implies that \algname\ may have reward performance degradation when using a smaller initial value of $h_D^0.$
One possible reason is that when the distance between the learned and baseline policies is large, using a small value of $h_D^0$ results in an inaccurate projection (\ie due to approximation errors).
This causes the policy to follow a zigzag path.
We leave the improvement of this in future work.

\begin{figure*}[t]
\vspace{-3mm}
\centering

\subfloat[Ant circle\label{subfig:ac}]{\begin{tabular}[b]{@{}c@{}}%
\includegraphics[width=0.33\linewidth]{figure/exp_2/NumCost_ac_overallPerformance_v2_init_hp_algo.png}%
\includegraphics[width=0.33\linewidth]{figure/exp_2/Reward_ac_overallPerformance_v2_init_hp_algo.png}%
\includegraphics[width=0.33\linewidth]{figure/exp_2/NumDemo_ac_overallPerformance_v2_init_hp_algo.png}%
\end{tabular}}%

\subfloat[Car-racing\label{subfig:cr}]{\begin{tabular}[b]{@{}c@{}}%
\includegraphics[width=0.33\linewidth]{figure/exp_2/NumCost_cr_initial_hp.png}%
\includegraphics[width=0.33\linewidth]{figure/exp_2/Reward_cr_initial_hp.png}%
\includegraphics[width=0.33\linewidth]{figure/exp_2/NumDemo_cr_initial_hp.png}%
\end{tabular}}%

\vspace{+1mm}

\includegraphics[width=0.7\linewidth]{figure/exp_2/legend_differentHd.png}
\vspace{-2mm}

\caption{
The undiscounted constraint cost,
the discounted reward, and
the undiscounted divergence cost
over policy updates for the tested algorithms and tasks.
The solid line is the mean and the shaded area is the standard deviation over 5 runs.
We observe that the initial value of $h_D^0$ does not affect the reward and the cost performance significantly.
(Best viewed in color.)
}
\label{fig:appendix_initialPriorConstraintThreshold}
\vspace{-3mm}
%\end{mdframed}
\end{figure*}

\section{Human Policies}
\label{appendix:human_policy}
We now describe the procedure for collecting human demonstration data in the car-racing task.
A player uses the right key, left key, up key and down key to control the direction, acceleration, and brake of the car. 
The human demonstration data contain the display of the game (\ie the observed state), the actions, and the reward.
We collect 20 minutes of demonstration data.
A human player is instructed to stay in the lane but does not know the cost constraint.
This allows us to test whether \algname\ can safely learn from the baseline policy which need not satisfy the cost constraints.
We then use an off-policy algorithm (DDPG) trained on the demonstration data to get the baseline human policy.
Since the learned baseline human policy does not interact with the environment, its reward performance cannot be better than the human performance.
Fig. \ref{fig:cr_human} shows the procedure.

\paragraph{Implementation Details of DDPG.} 
We use DDPG as our off-policy algorithm. 
We use a convolutional neural network with two convolutional operators of size 24 and 12 followed by a dense layer of size (32, 16) to represent a Gaussian policy. 
A Q function shares the same architecture of the policy.
The learning rates of the policy and Q function are set to $10^{-4}$ and $10^{-3},$ respectively.
%
%The remaining hyperparameters can be found in ~\url{https://sites.google.com/view/spaceneurips}.

\begin{figure*}[t]
\centering
\includegraphics[scale=0.25]{figure/cr_human.png}
\caption{
Procedure for getting a baseline human policy. 
We ask a human to play the car-racing game.
He/She does not know the cost constraint.
The trajectories (\ie display of the game, the action, and the reward) are then stored.
A human policy is obtained by using an off-policy algorithm (DDPG) trained on the trajectories.
}
\label{fig:cr_human}
\end{figure*}

\iffalse
\section{Comparison between PCPO \cite{yang2020projection} and CPO \cite{achiam2017constrained}} Fig. \ref{fig:pcpo_cpo}.

\begin{figure*}[t]
\vspace{-3mm}
\centering
\subfloat[PCPO \cite{yang2020projection}]{
\includegraphics[width=0.23\linewidth]{figure/pcpo.pdf}}
\subfloat[CPO \cite{achiam2017constrained}]{
\includegraphics[width=0.23\linewidth]{figure/cpo.pdf}}
\caption{Update procedures of for PCPO and CPO. 
}
\vspace{-3mm}
\label{fig:pcpo_cpo}
\vspace{-3mm}
%\end{mdframed}
\end{figure*}
\fi

\section{The Machine Learning Reproducibility Checklist (Version 1.2, Mar.27 2019)}
\label{appendix:sec:reproduce}
For all models and algorithms presented, indicate if you include\footnote{Here is a link to the list: \url{https://www.cs.mcgill.ca/~jpineau/ReproducibilityChecklist.pdf}.}:
\begin{itemize}
\item A clear description of the mathematical setting, algorithm, and/or model:
    \begin{itemize}
         \item \textbf{Yes}, please see the problem formulation in Section \ref{sec:preliminaries}, the update procedure for \algname\ in Section \ref{sec:implementation}, and the architecture of the policy in Section \ref{subsec:appendix_details}.
    \end{itemize}
\item An analysis of the complexity (time, space, sample size) of any algorithm:
    \begin{itemize}
        \item \textbf{Yes}, please see the implementation details in Section \ref{subsec:appendix_details}.
    \end{itemize}
\item A link to a downloadable source code, with specification of all dependencies, including external libraries:
    \begin{itemize}
        \item \textbf{Yes}, please see the implementation details in Section \ref{subsec:appendix_details}.
    \end{itemize}
\end{itemize}
For any theoretical claim, check if you include:
\begin{itemize}
\item A statement of the result:
    \begin{itemize}
        \item \textbf{Yes}, please see Section \ref{sec:model} and Section \ref{subsec:p2cpoConvergence}.
    \end{itemize}
\item A clear explanation of any assumptions:
    \begin{itemize}
        \item \textbf{Yes}, please see Section \ref{sec:model} and Section \ref{subsec:p2cpoConvergence}.
    \end{itemize}
\item A complete proof of the claim:
    \begin{itemize}
        \item \textbf{Yes}, please see Section~\ref{appendix:sec:theorem:h_D}, Section \ref{appendix:proof_update_rule_1},
        and Section \ref{appendix:sec:converge}.
    \end{itemize}
\end{itemize}
For all figures and tables that present empirical results, indicate if you include:
\begin{itemize}
\item A complete description of the data collection process, including sample size:
    \begin{itemize}
        \item \textbf{Yes}, please see Section \ref{subsec:appendix_details} for the implementation details.
    \end{itemize}    
\item A link to a downloadable version of the dataset or simulation environment:
    \begin{itemize}
        \item \textbf{Yes}, please see Section \ref{subsec:appendix_details} for the simulation environment.
    \end{itemize}  
\item An explanation of any data that were excluded, description of any pre-processing step:
    \begin{itemize}
        \item \textbf{It's not applicable.} This is because that data comes from simulated environments.
    \end{itemize}  

\item An explanation of how samples were allocated for training / validation / testing:
    \begin{itemize}
        \item \textbf{It's not applicable.} The complete trajectories (\ie data) is used for training. There is no validation set. Testing is performed in the form of online learning approaches.
    \end{itemize}  
    
\item The range of hyper-parameters considered, method to select the best hyper-parameter configuration, and specification of all hyper-parameters used to generate results:
    \begin{itemize}
        \item \textbf{Yes}, we randomly select five random seeds, and please see Section \ref{subsec:appendix_details} for the implementation details. 
    \end{itemize}  
    
\item The exact number of evaluation runs:
    \begin{itemize}
        \item \textbf{Yes}, please see Section \ref{subsec:appendix_details} for the implementation details. 
    \end{itemize}  

\item A description of how experiments were run:
    \begin{itemize}
        \item \textbf{Yes}, please see Section \ref{subsec:appendix_details} for the implementation details. 
    \end{itemize}  
    
\item A clear definition of the specific measure or statistics used to report results:
    \begin{itemize}
        \item \textbf{Yes}, please see Section \ref{sec:experiments}. 
    \end{itemize}

\item Clearly defined error bars:
    \begin{itemize}
        \item \textbf{Yes}, please see Section \ref{sec:experiments}. 
    \end{itemize}  

\item A description of results with central tendency (\eg mean) variation (\eg stddev):
    \begin{itemize}
        \item \textbf{Yes}, please see Section \ref{sec:experiments}. 
    \end{itemize}  

\item A description of the computing infrastructure used:
    \begin{itemize}
        \item \textbf{Yes}, please see Section \ref{subsec:appendix_details} for the implementation details. 
    \end{itemize}
\end{itemize}
